# Supplementary material for: Is the Gum Nebula an Important Interstellar Scattering Disk of Background Pulsars?
Source: arXiv:2410.08628 source file (2024-10-11)
Supplement: Supplementary file 1 [file supplement.pdf]

# Appendix

Supplemental materials for the paper "Is the Gum Nebula an Important Interstellar Scattering Disk of Background Pulsars?". All integration times are 30 s. The frequency resolution is 1.95 MHz at 8.60 GHz. At 2.25 GHz, the frequency resolution is 0.97 MHz on MJDs 59168.83, 59206.66, 59243.58, and 59293.46. On other dates, the frequency resolution was 0.24 MHz.

## S1. Dynamic spectrum plots

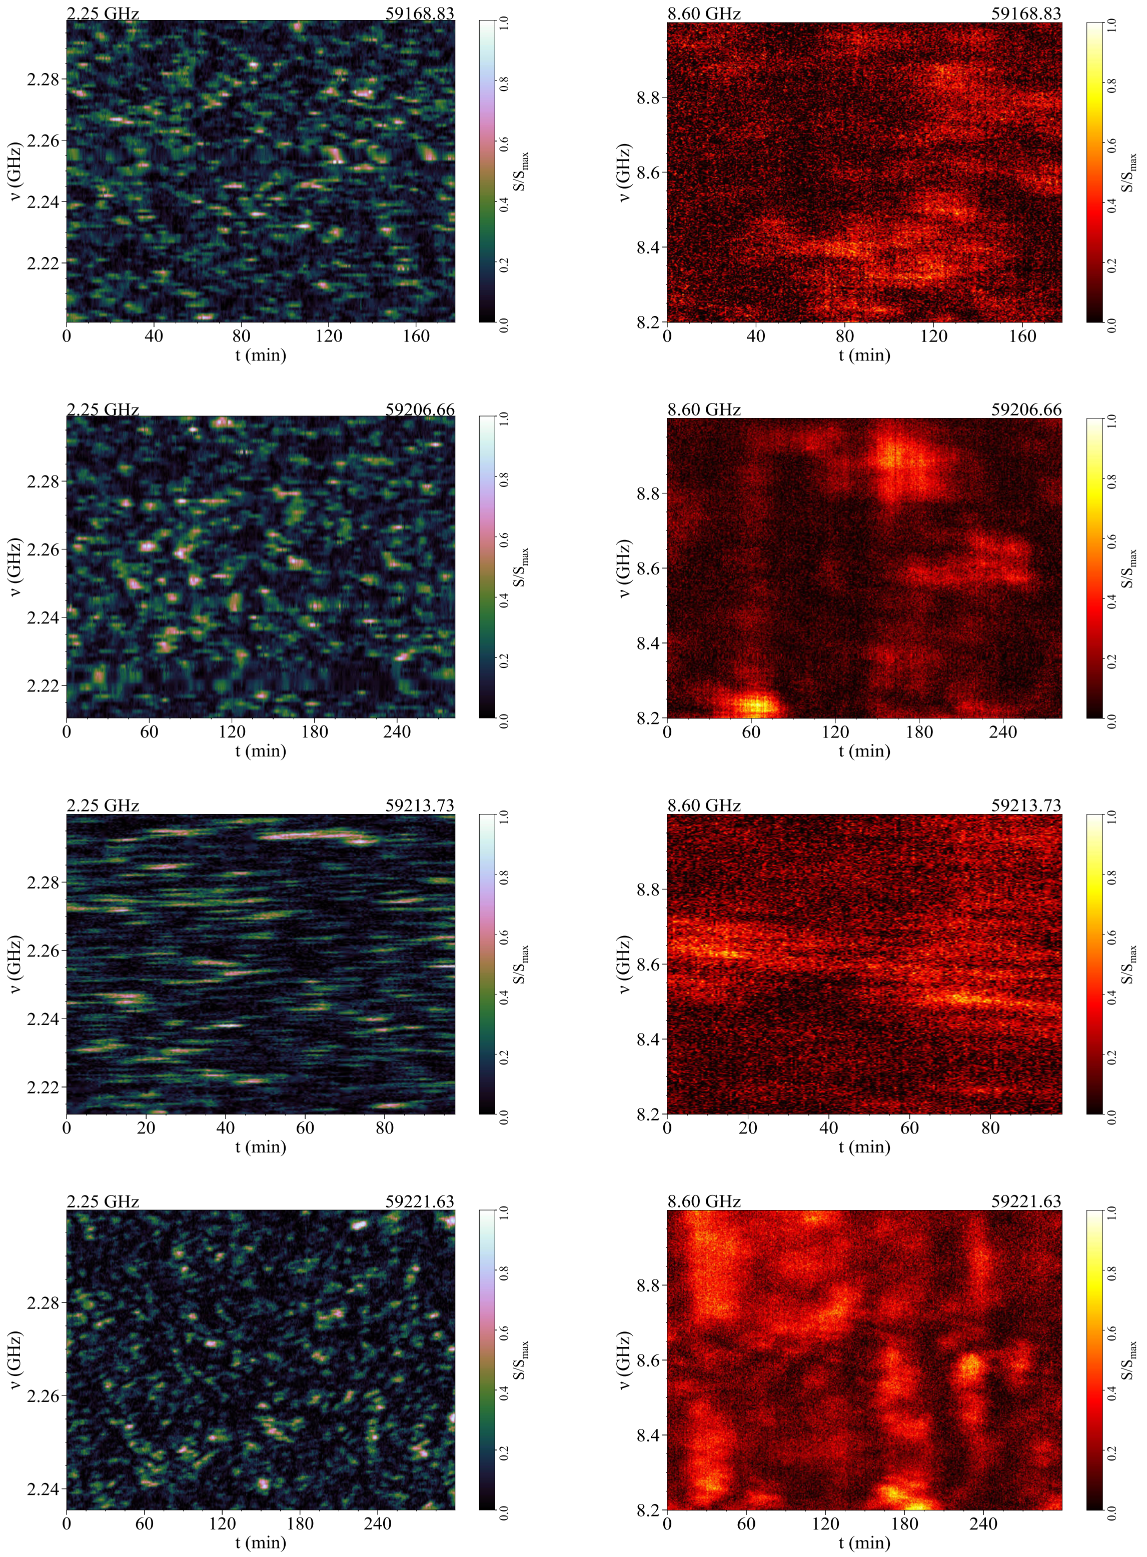


**Fig. S1** The dynamic spectrum plots for the 2.25 GHz (cube-helix style) and 8.60 GHz (hot style) observations of PSR B0740-28. The observed flux density is linearly scaled with the brightness of the corresponding pixel.

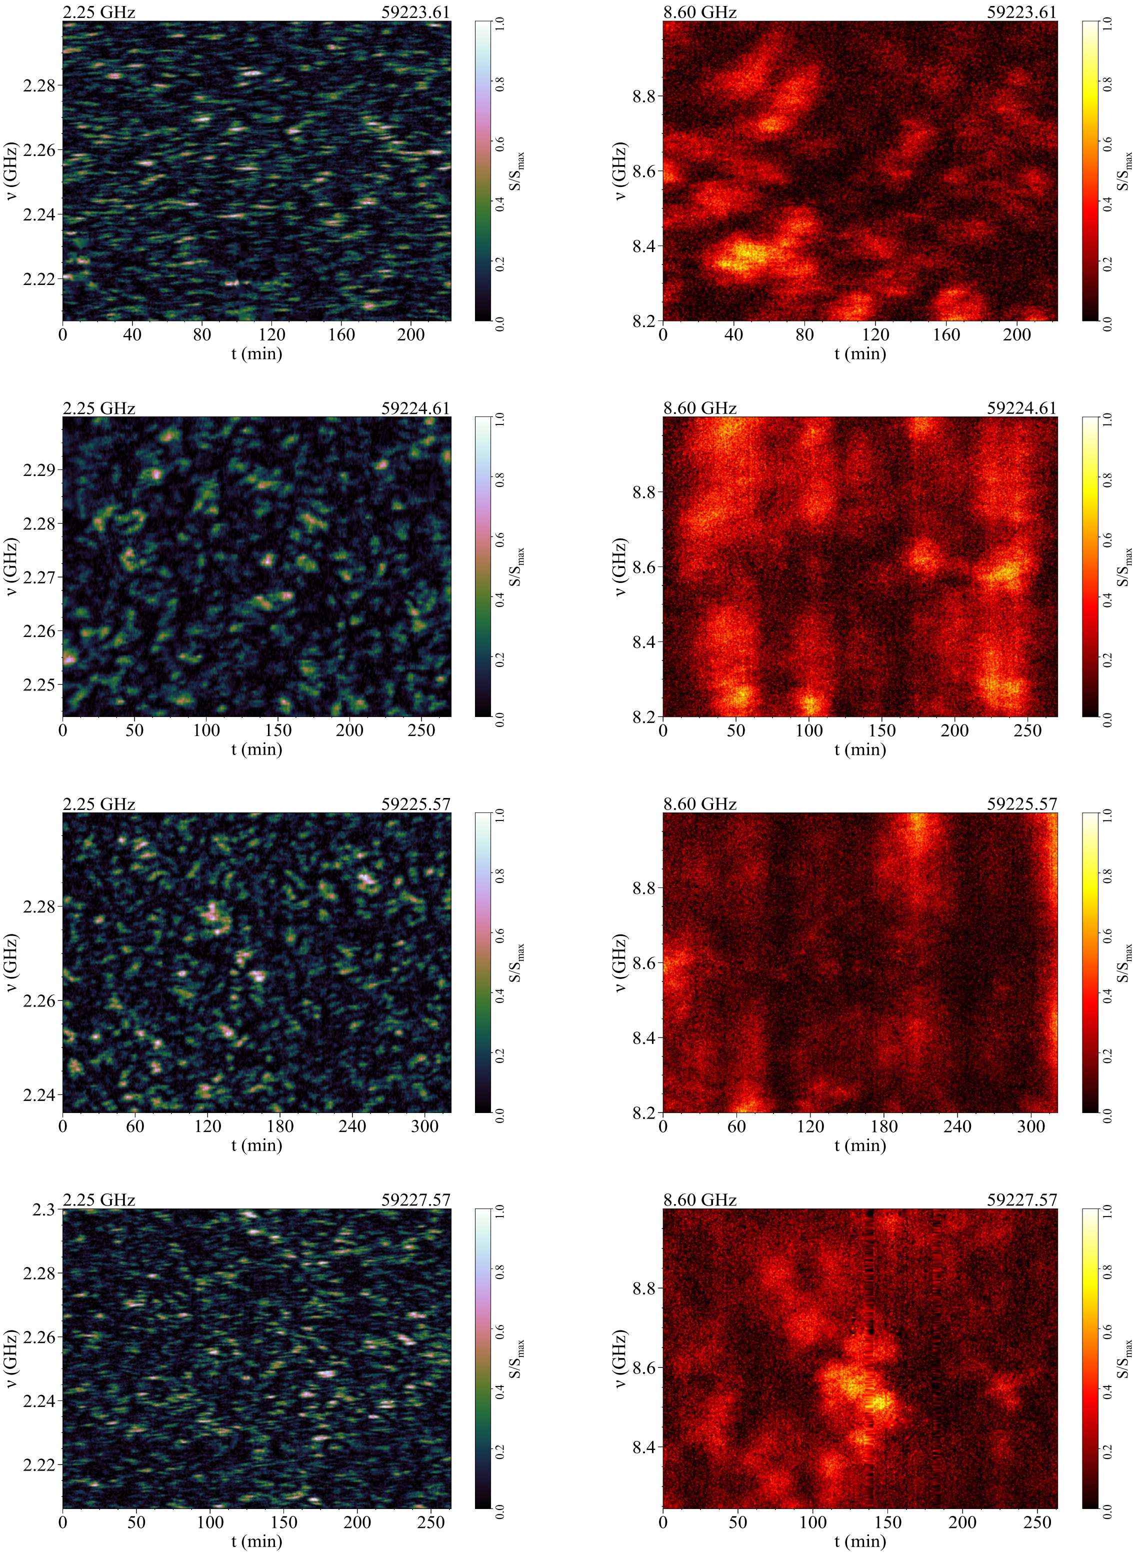


**Fig. S1** -continued

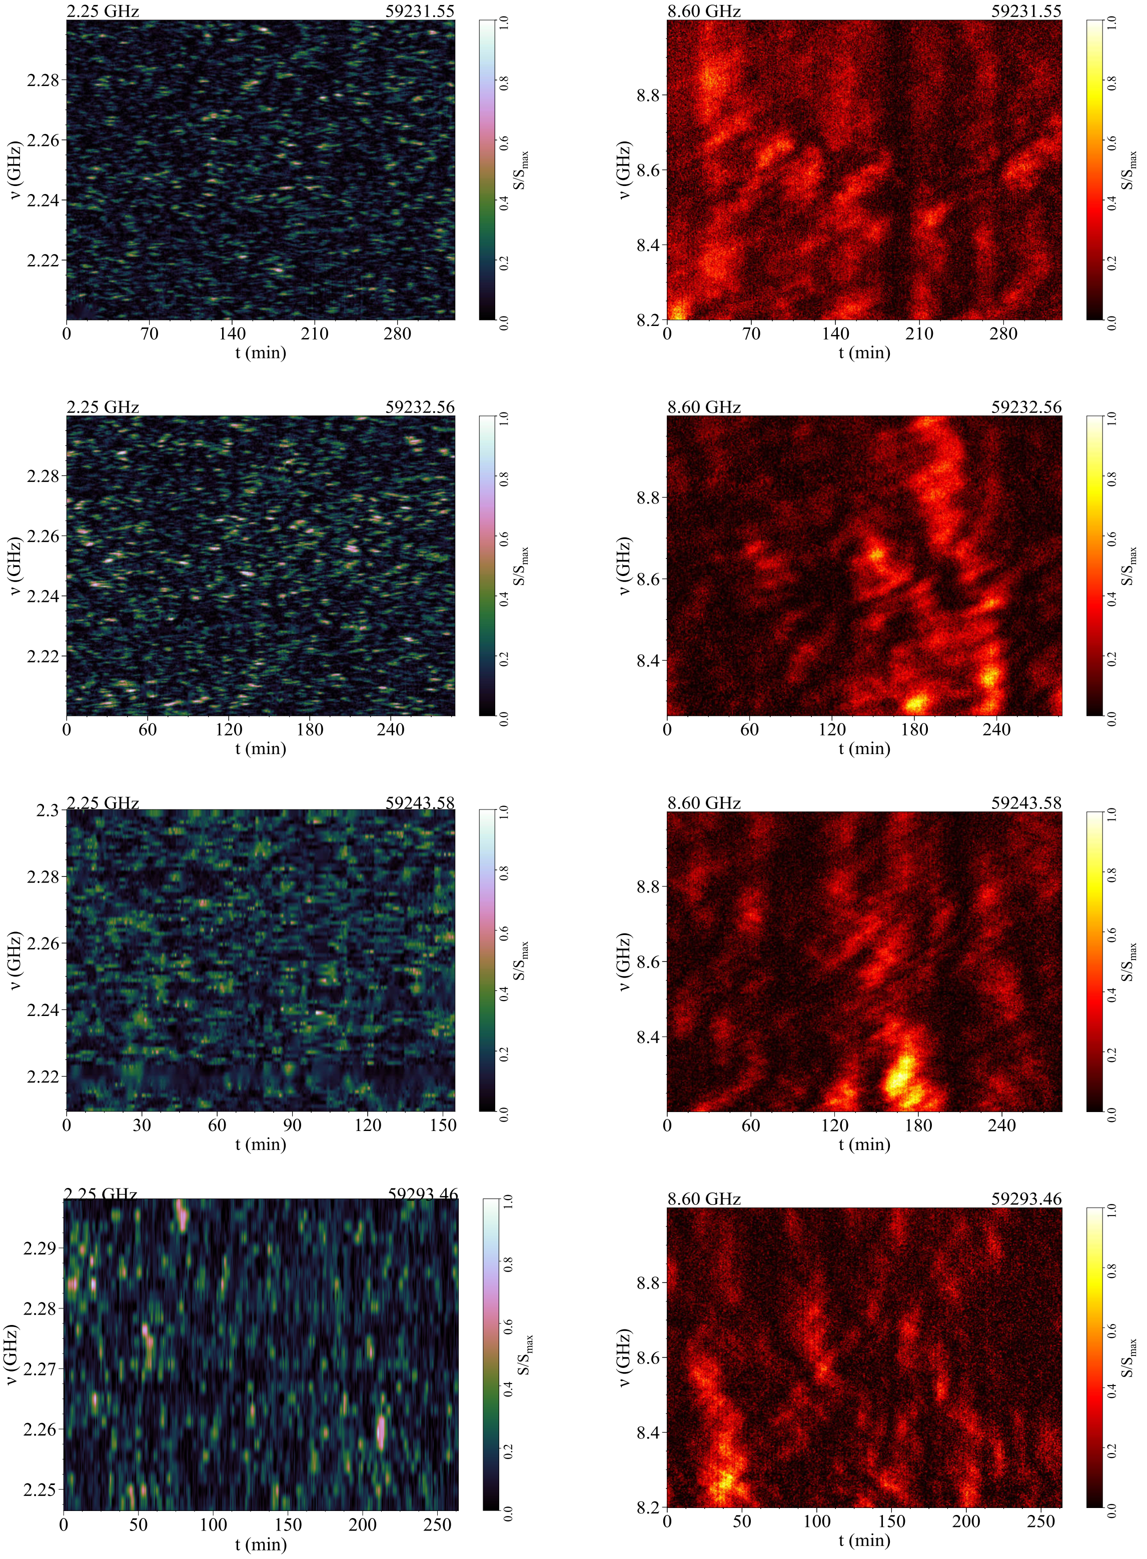


**Fig. S1** -continued

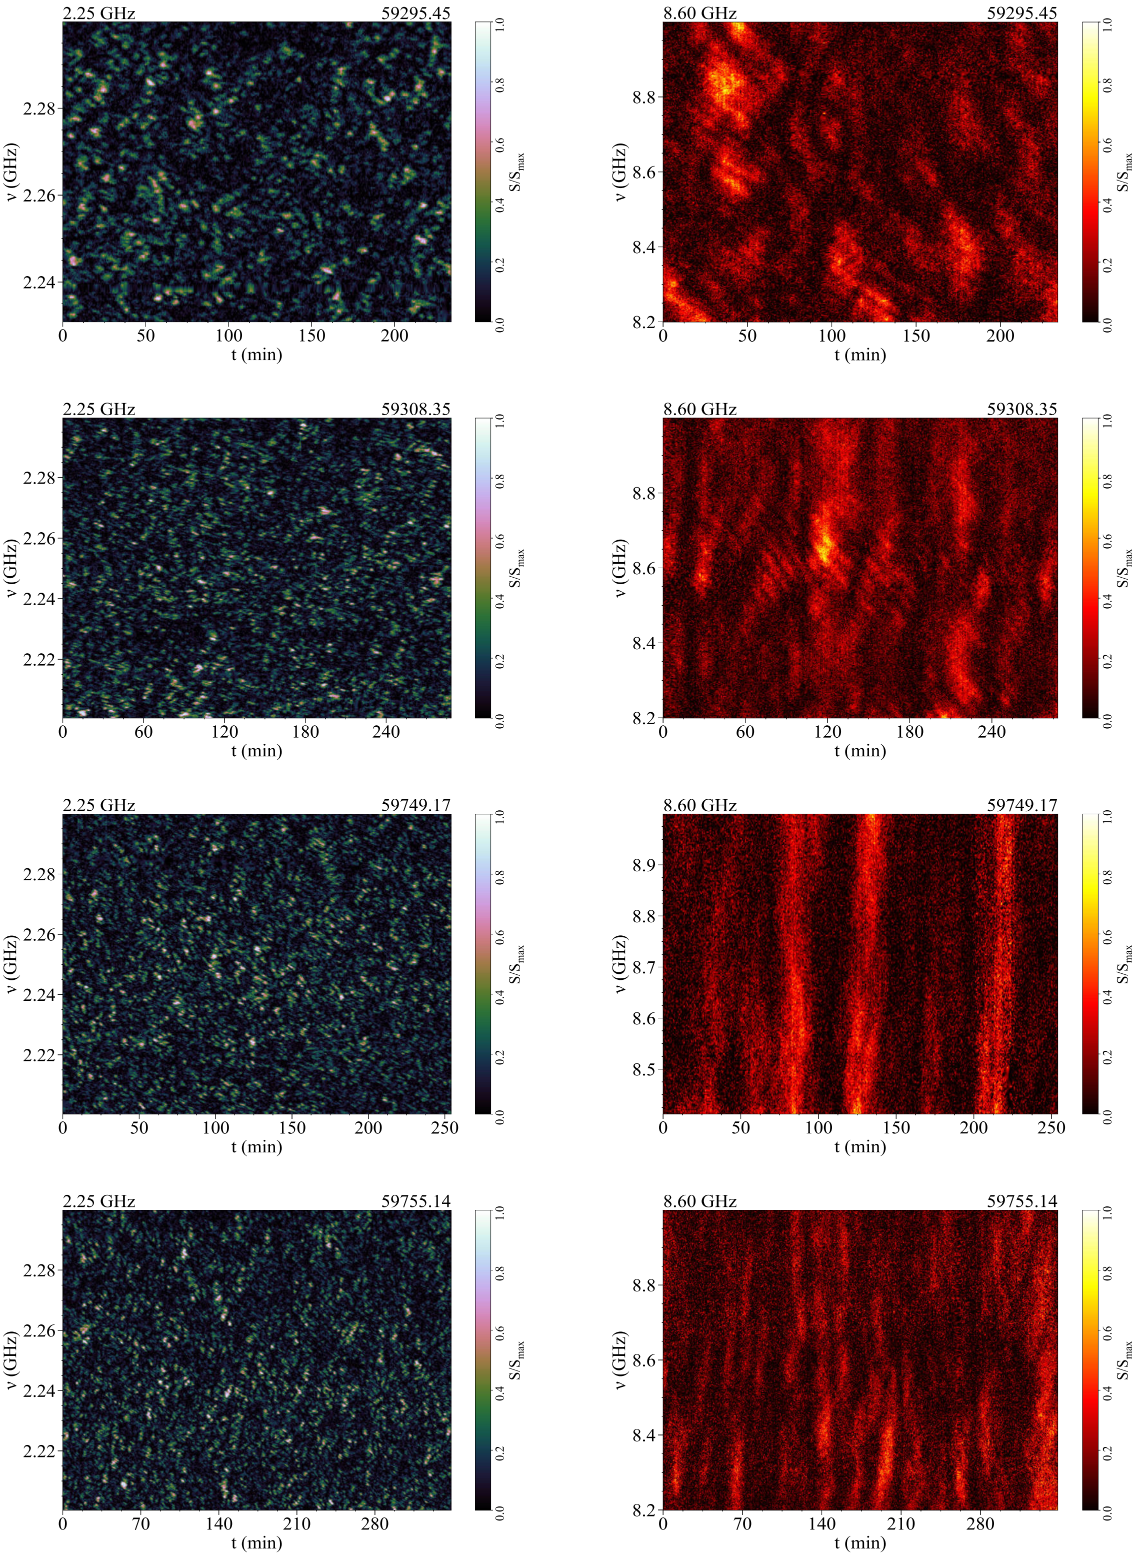


**Fig. S1** -continued

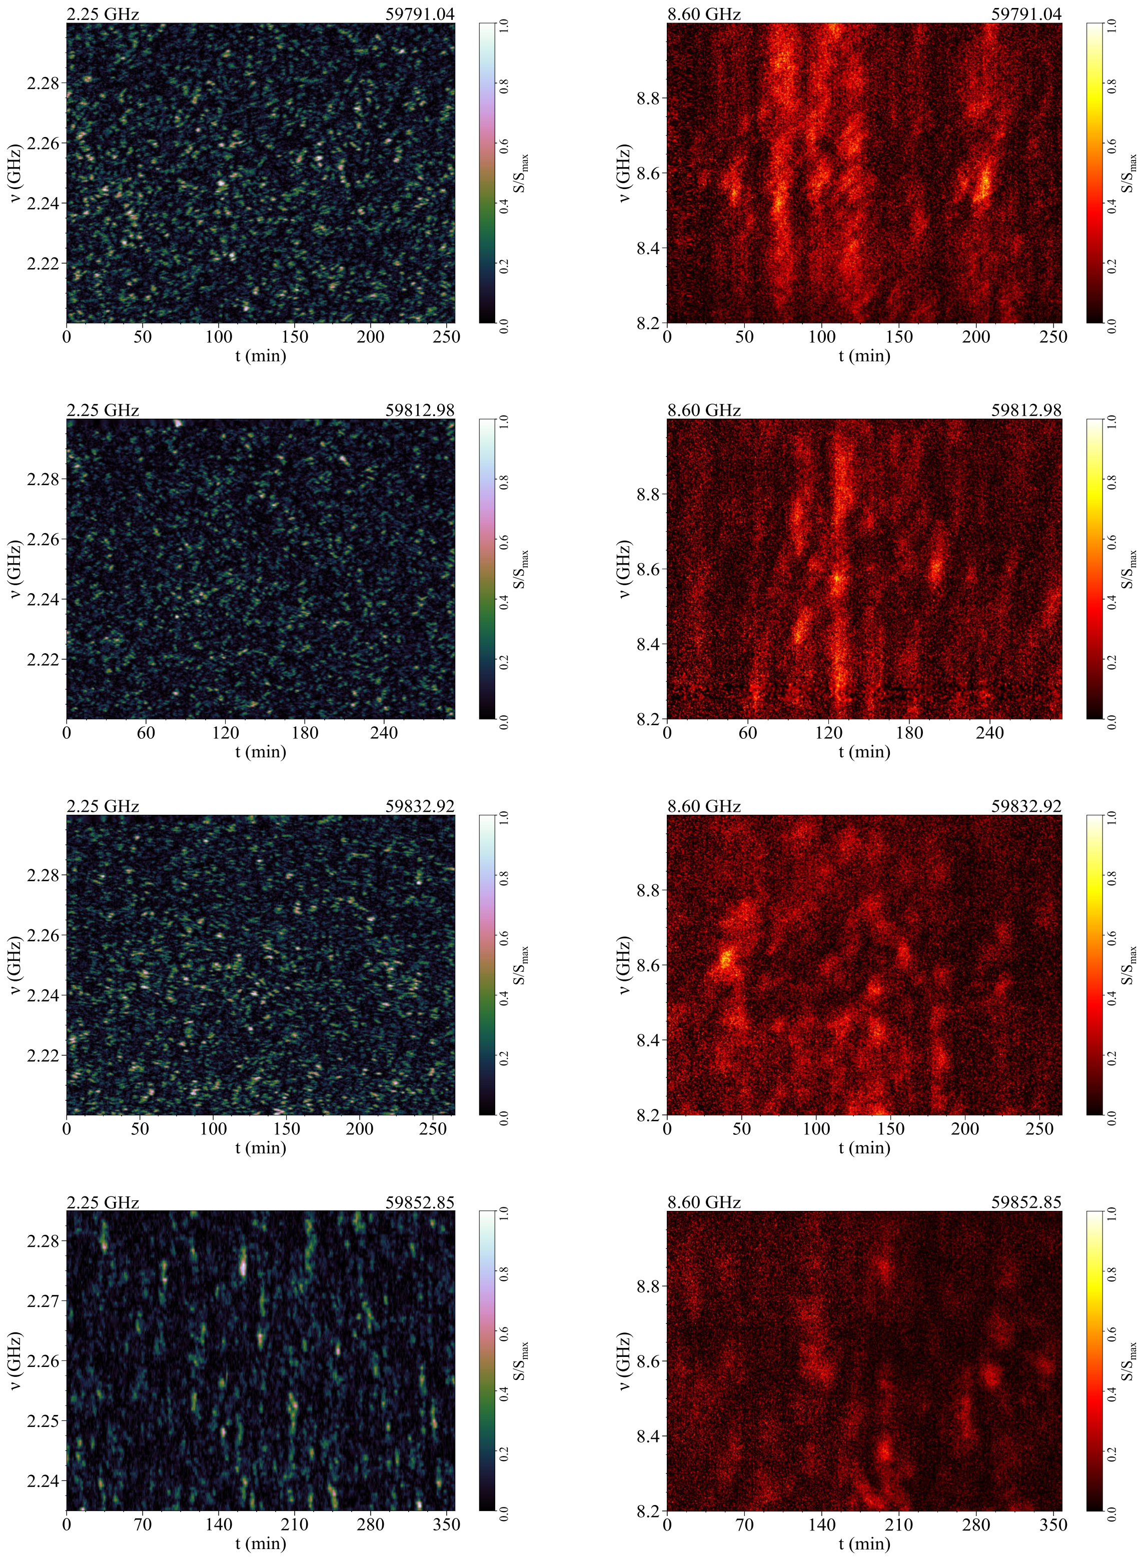


**Fig. S1** -continued

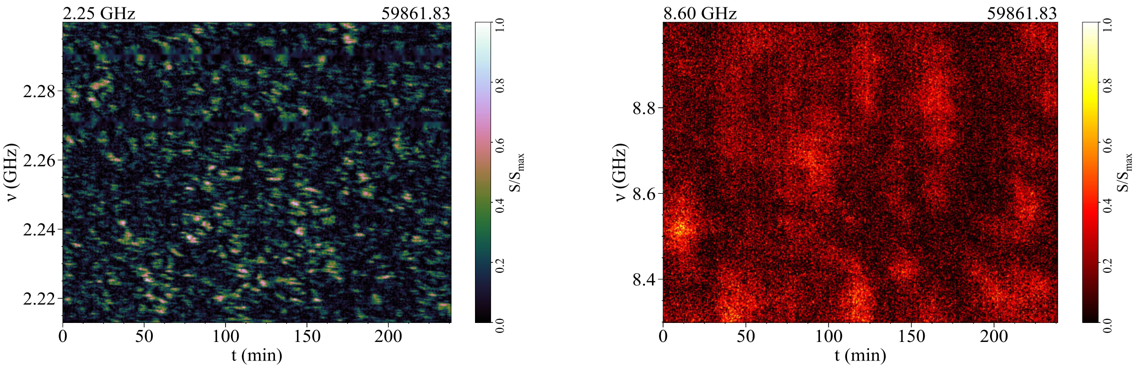


**Fig. S1** -continued

## S2. The two-dimensional auto covariance function (2D-ACF) plots

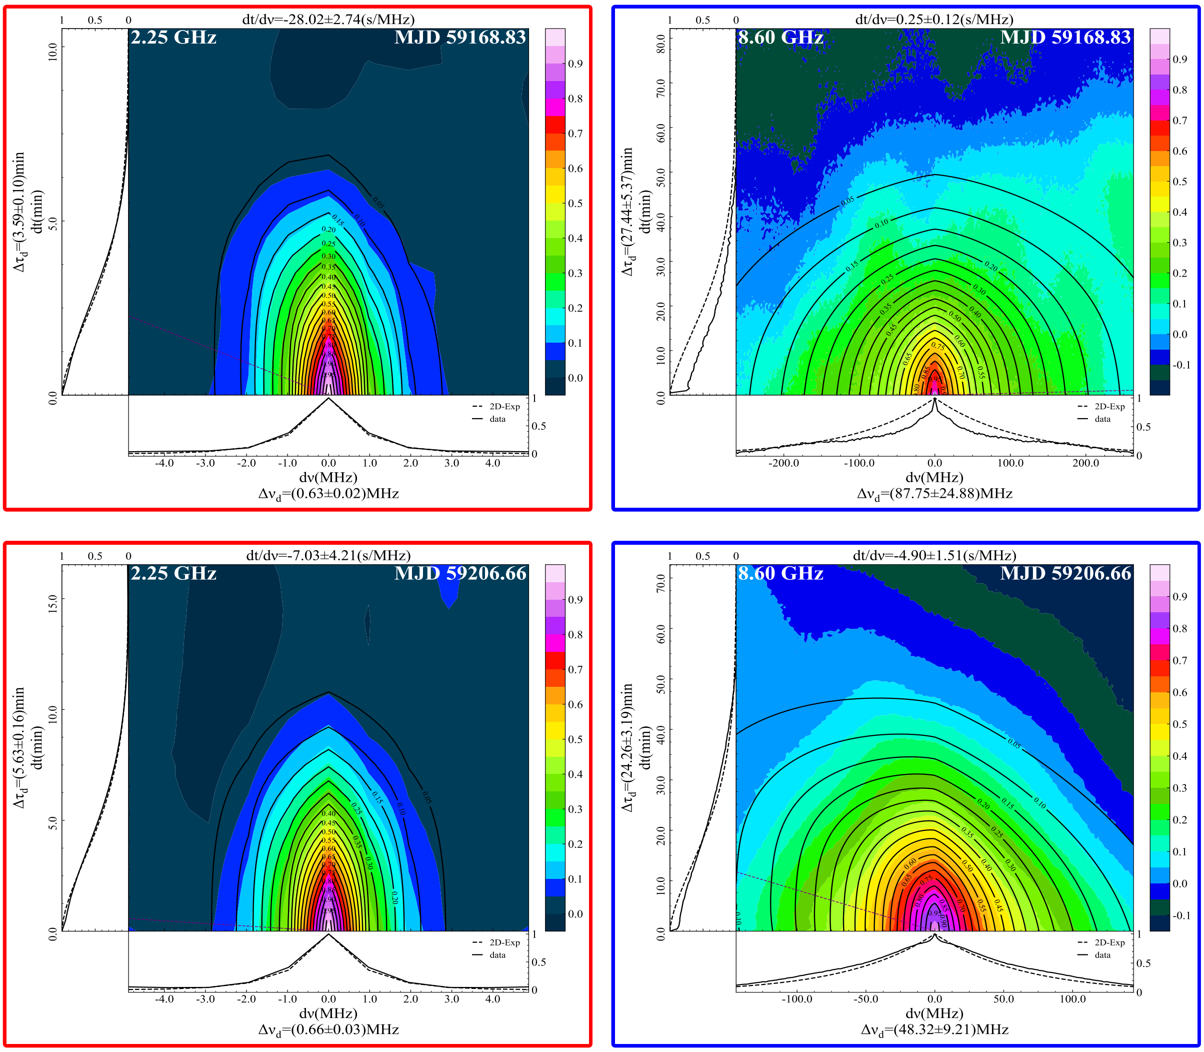


**Fig. S2** The normalizing 2D-ACF and the 2D-Exponential form function fitting results are shown in the central sub-panels. Their white noise peak at (0,0) has been smoothed. Normalizing 2D-ACFs are the color filled contour and scaled with a color bar on the right, while black curves are 2D-Exponential form function fitting results, respectively. The major axis for each best-fitted Exponential form function is also plotted with the purple dashed line. In the bottom and left sub-panels, the solid curves are the 1D-ACF results at zero time and frequency lag, respectively. Meanwhile, curves for the best-fitted $\Delta\nu_d$ and $\Delta\tau_d$ are shown with dashed lines correspondingly.

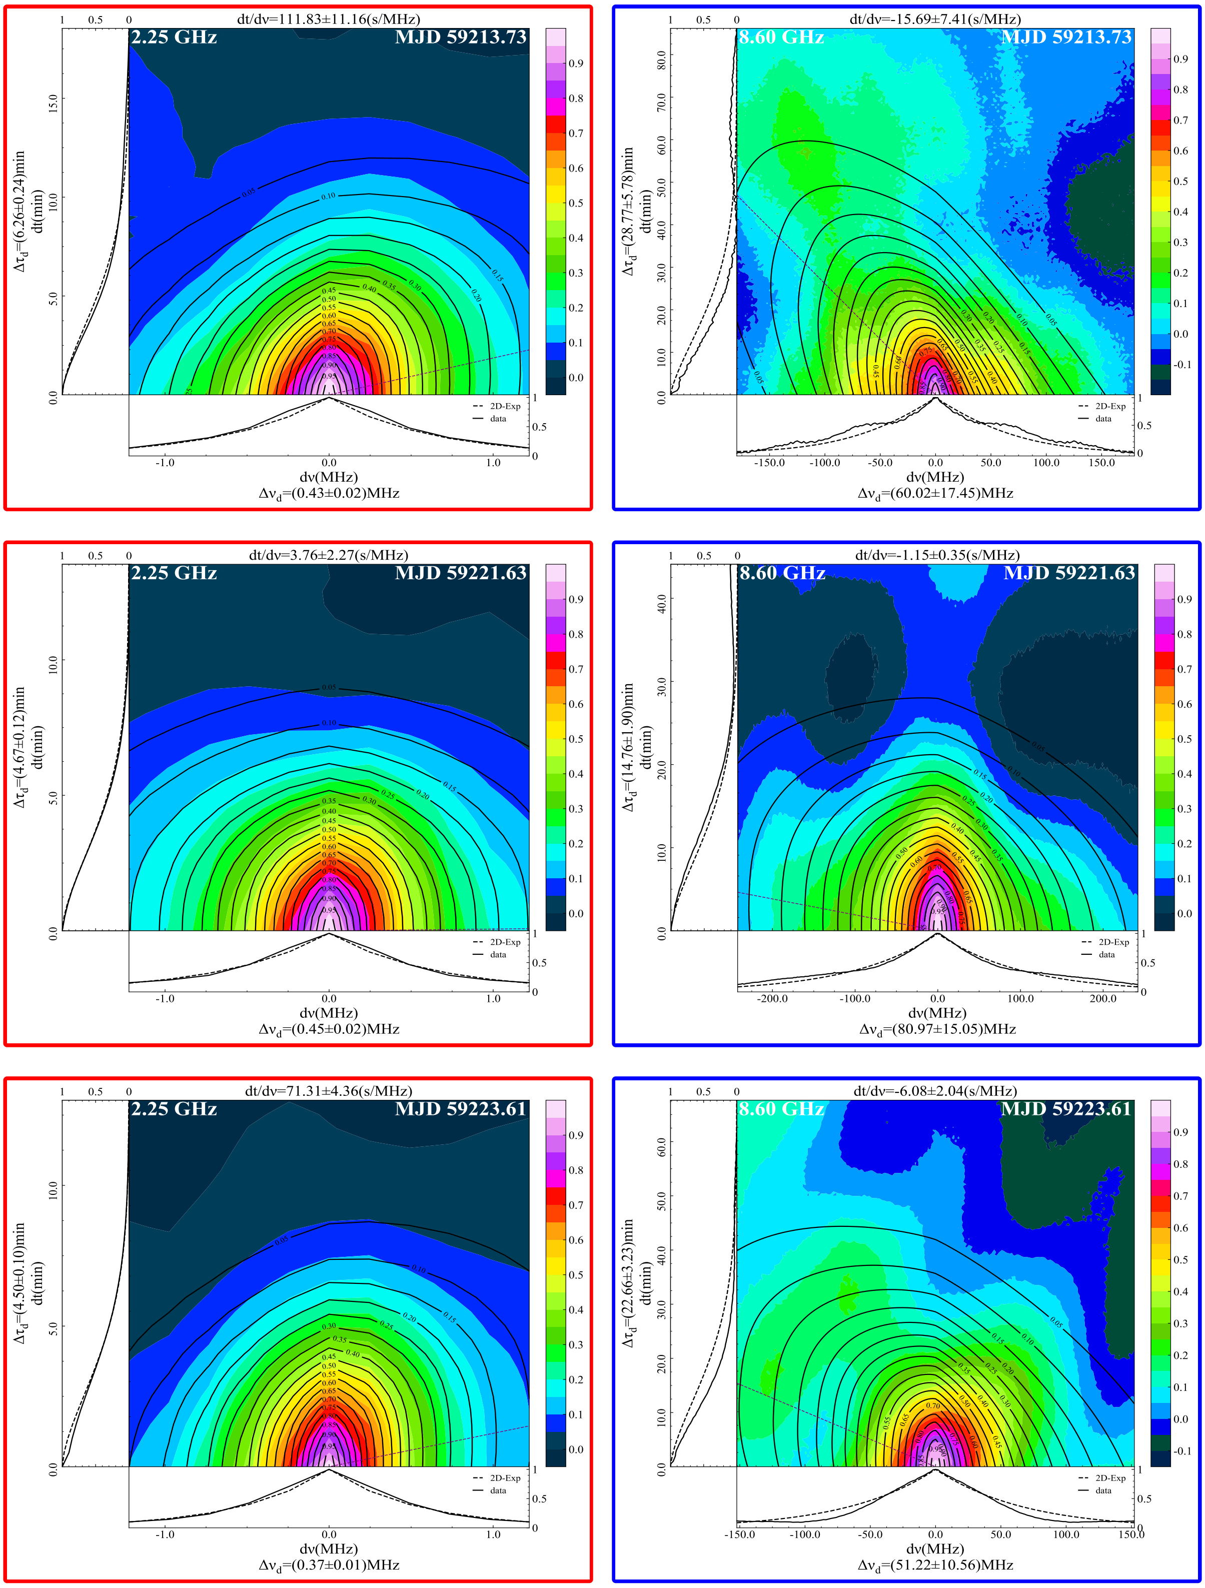


**Fig. S2** -continued

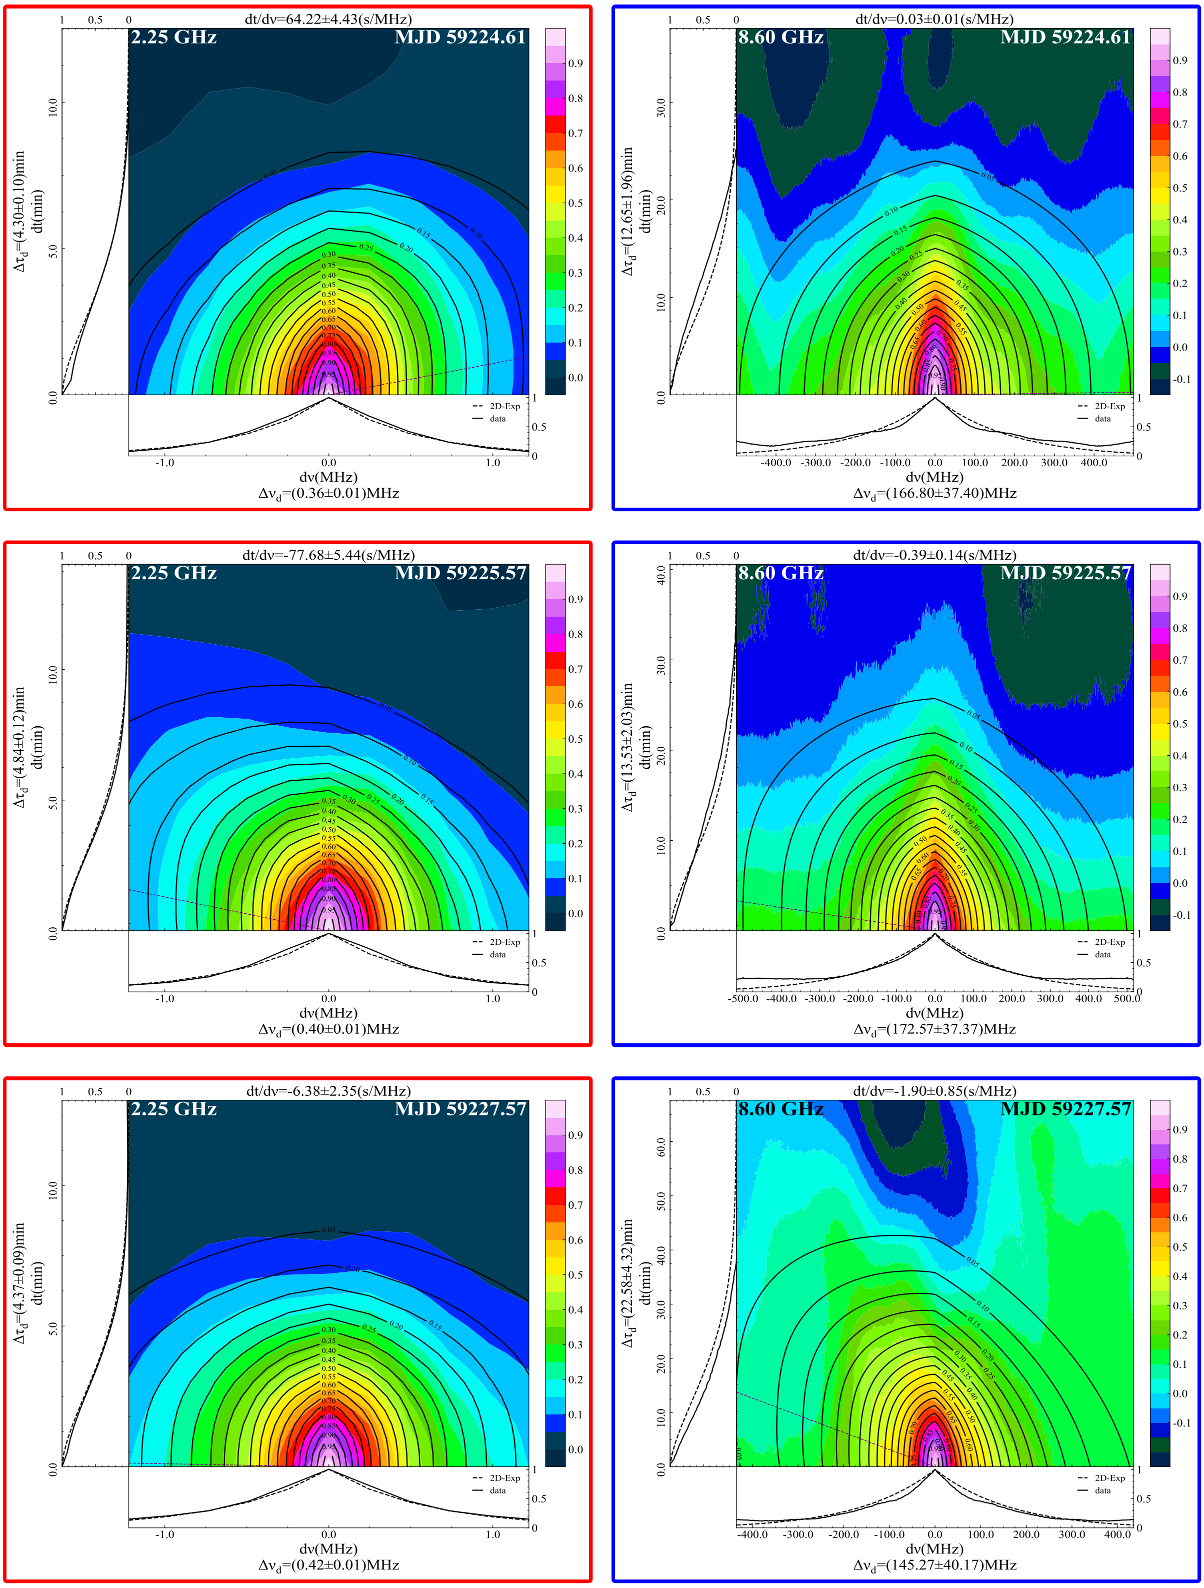


**Fig. S2** -continued

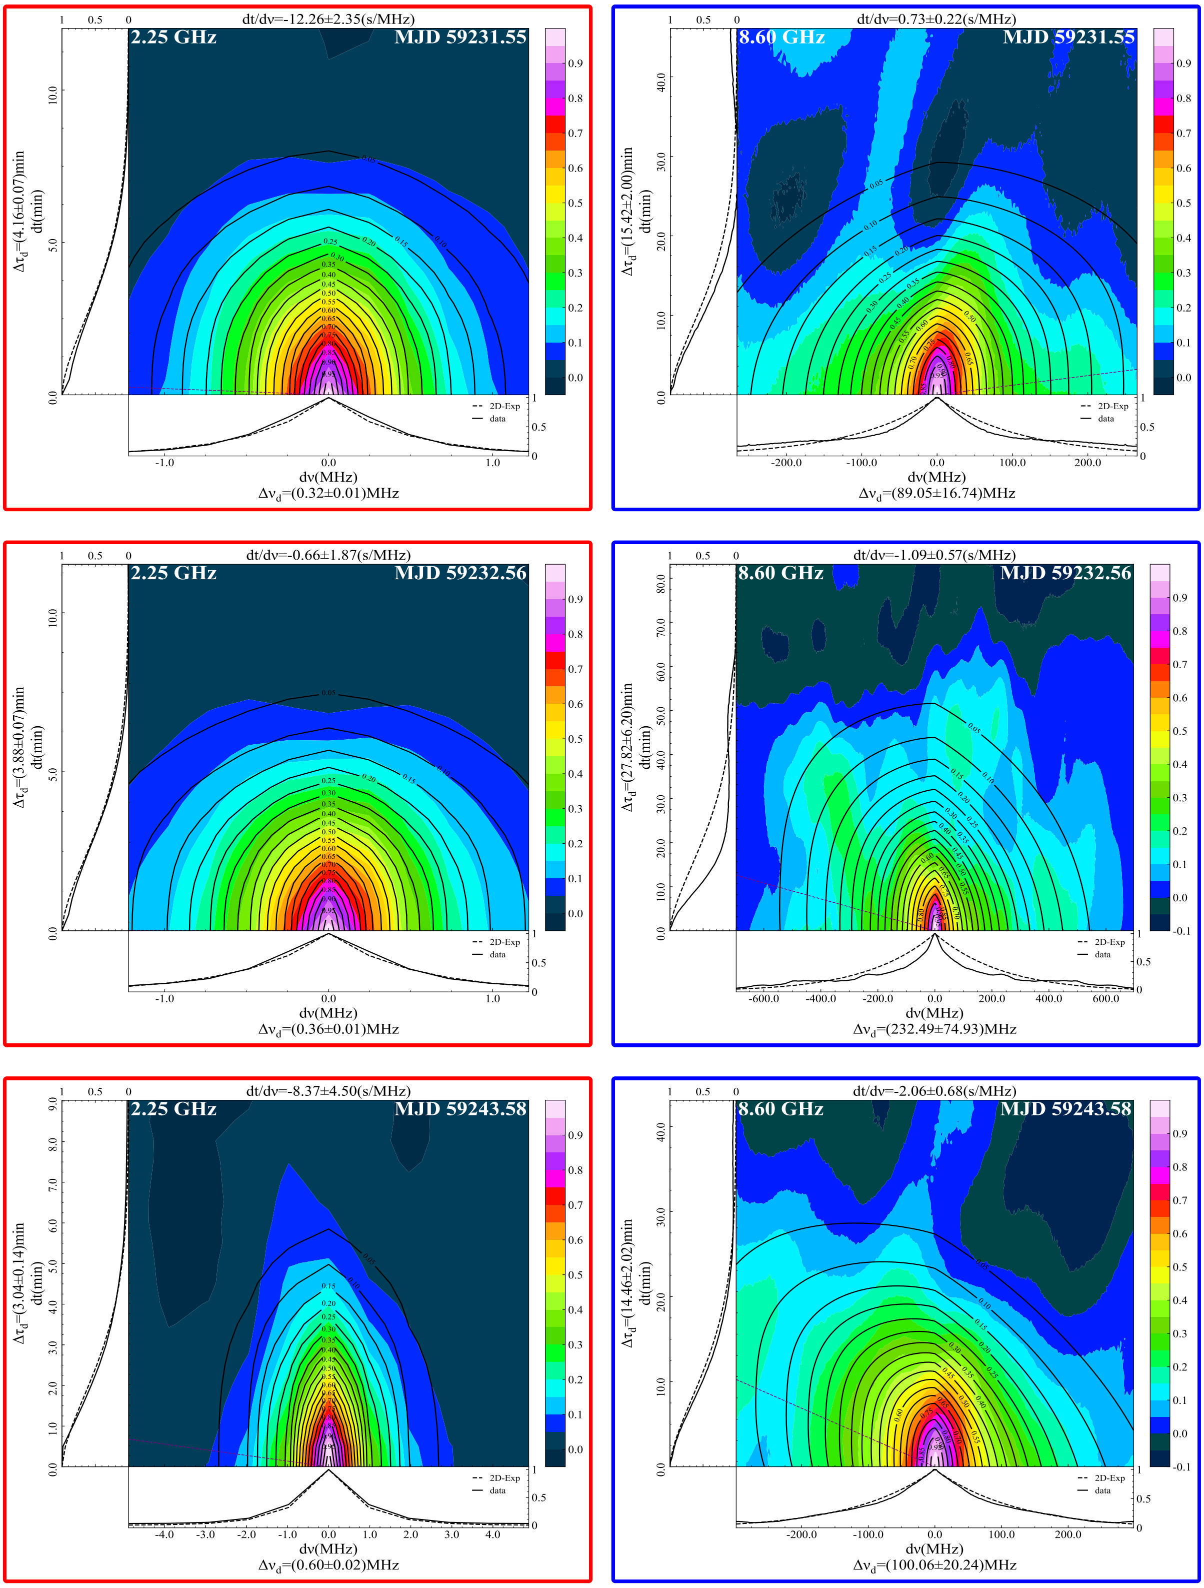


**Fig. S2** -continued

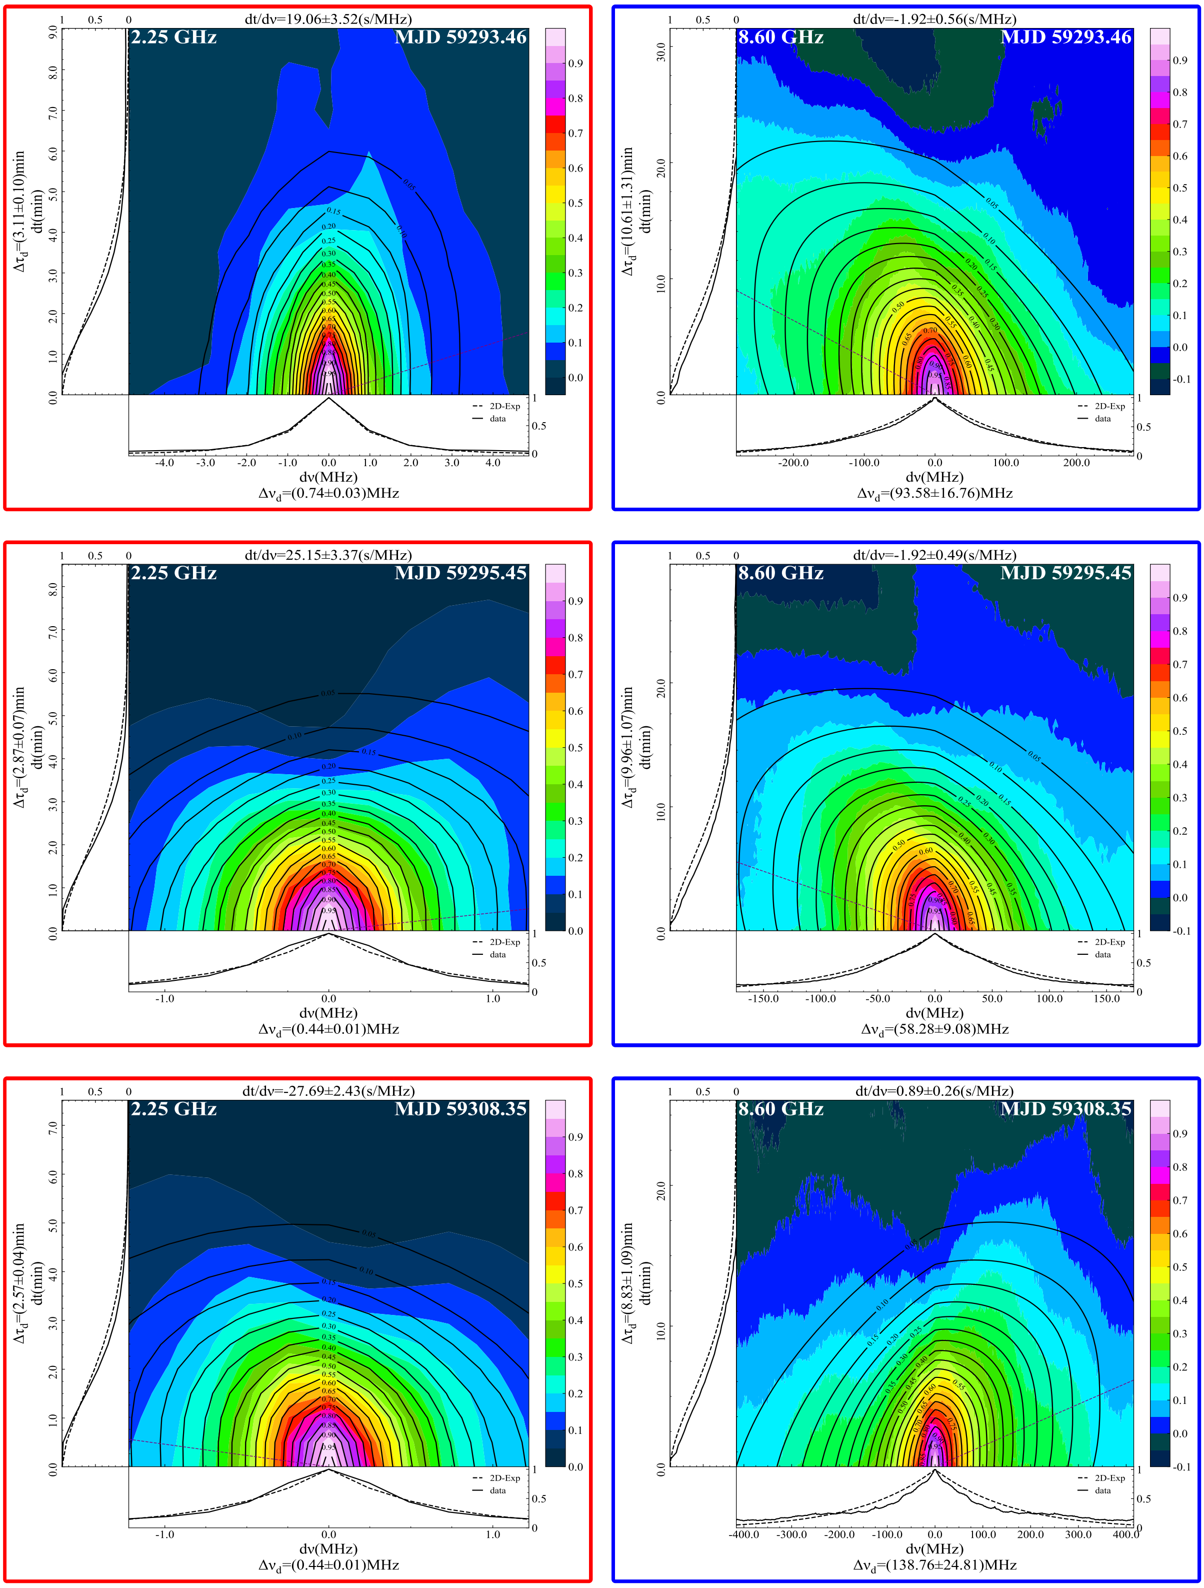


**Fig. S2** -continued

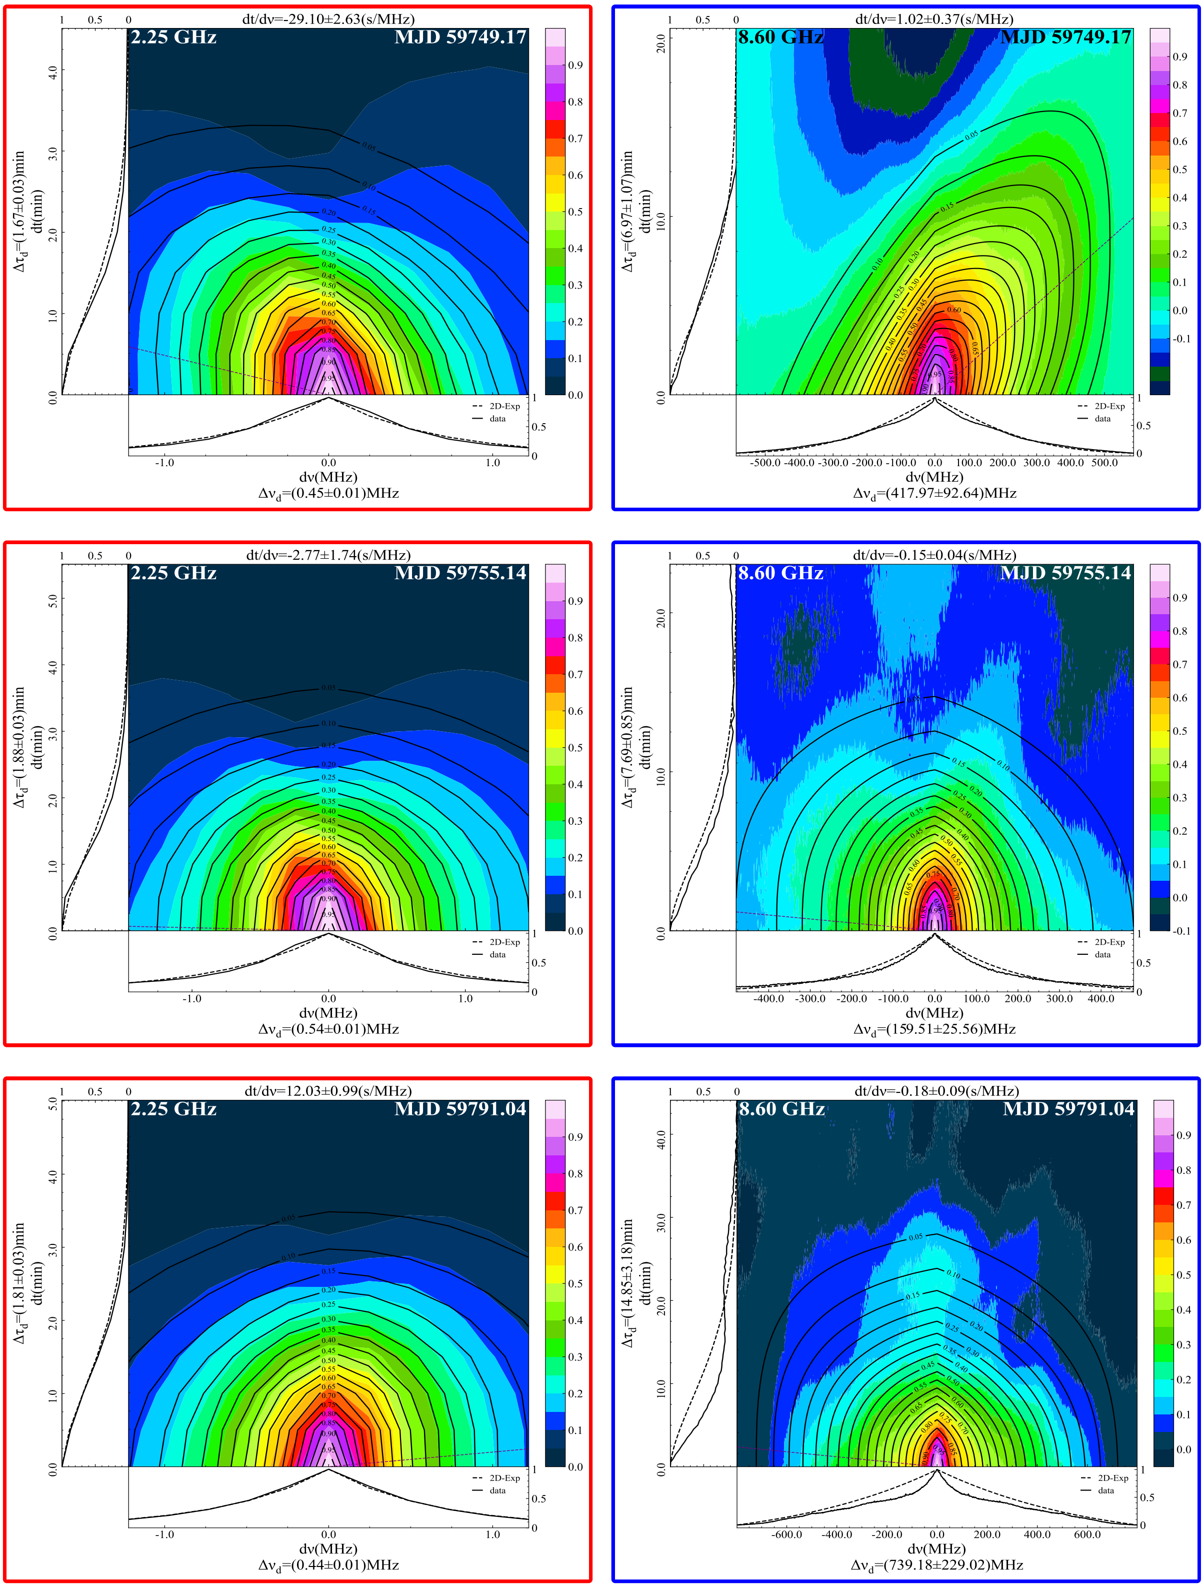


**Fig. S2** -continued

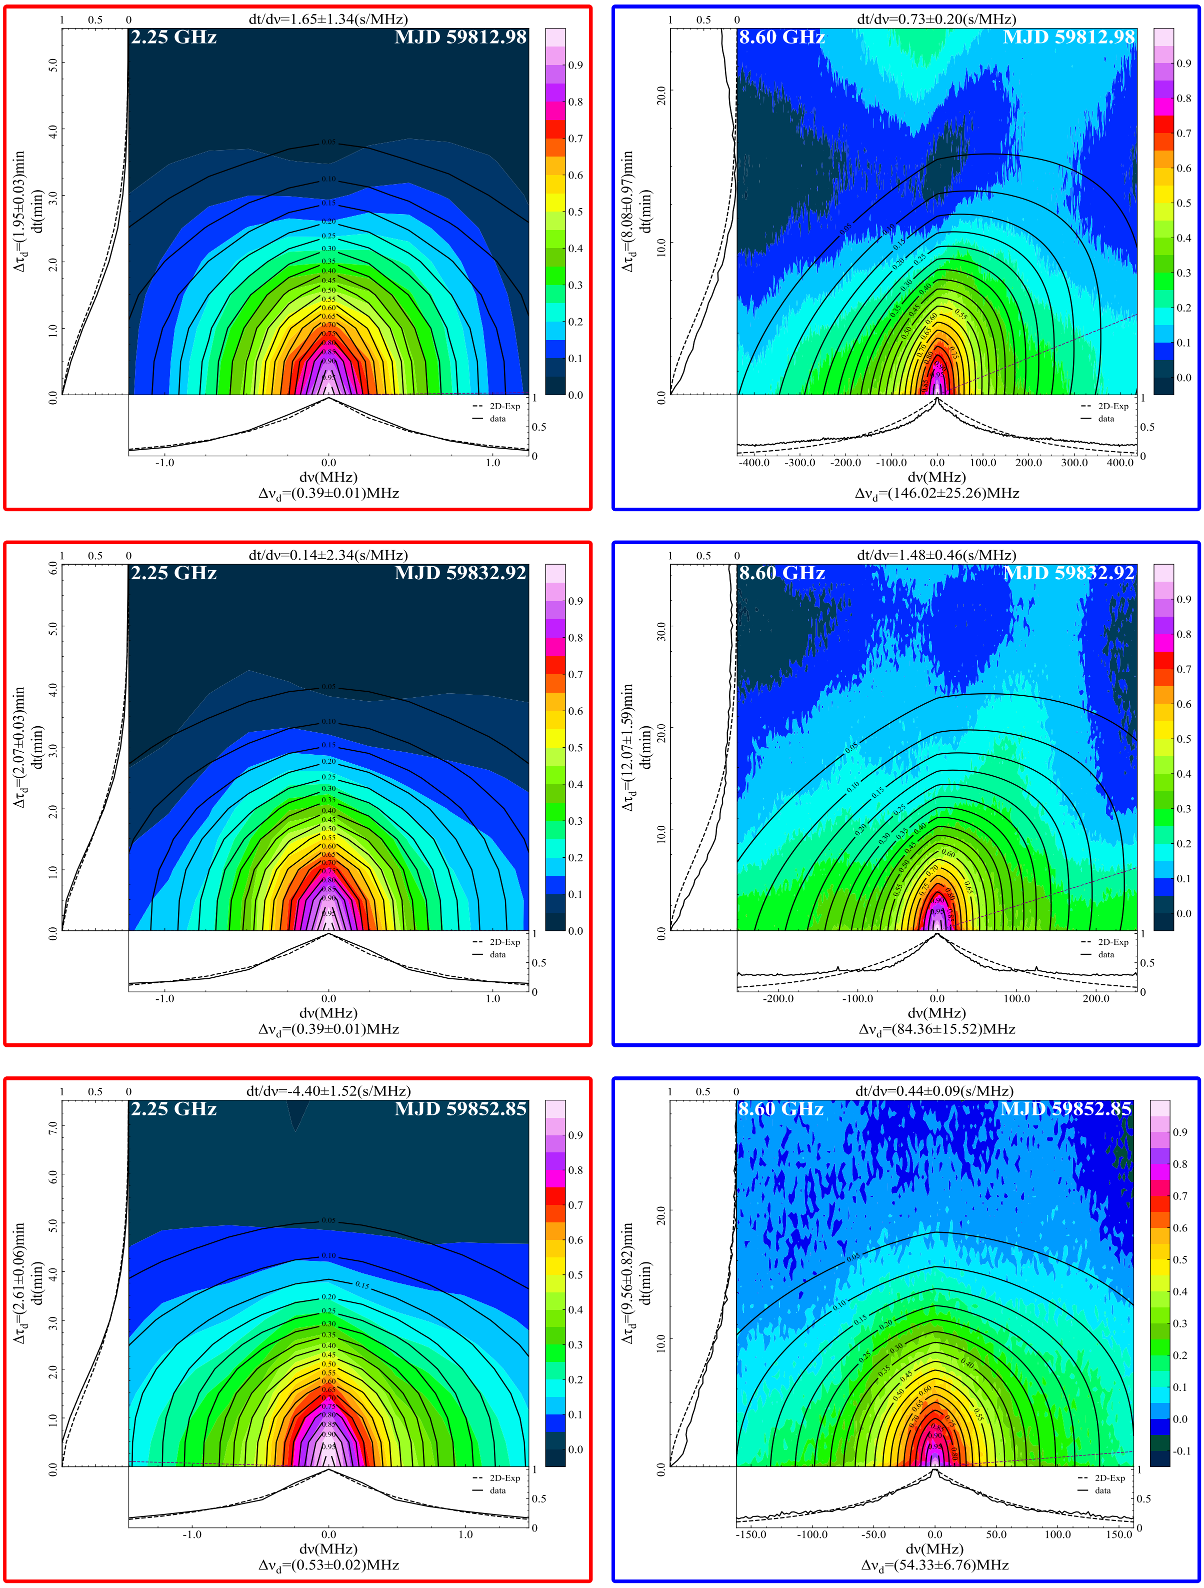


**Fig. S2** -continued

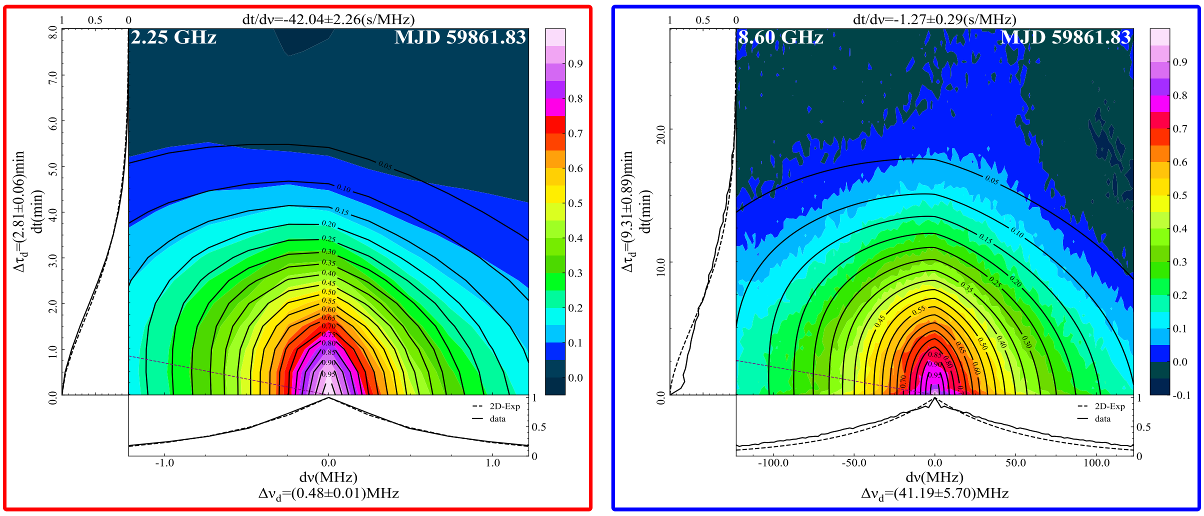


**Fig. S2** -continued

## S3. The secondary spectrum plots

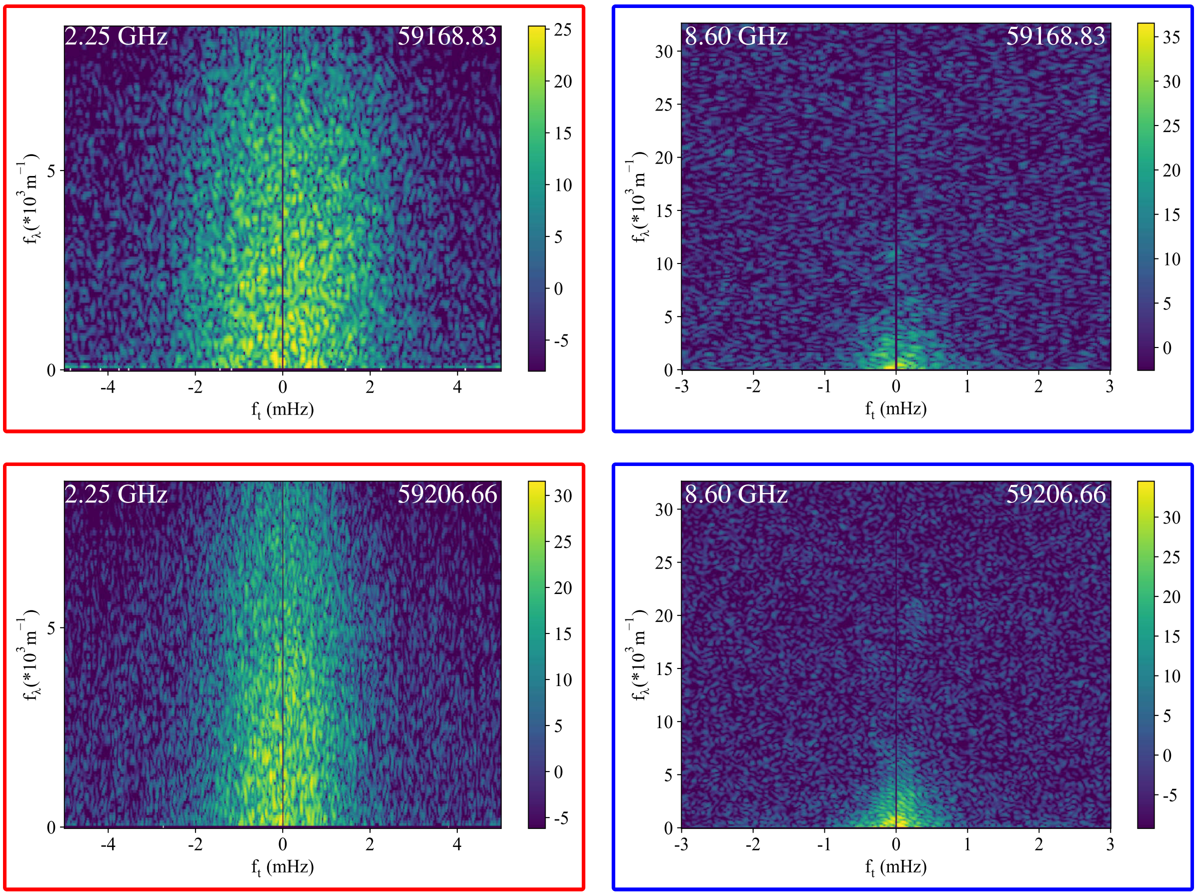


**Fig. S3** The secondary spectrum plots on a logarithmic scale for the 2.25 GHz (in red boxes) and 8.60 GHz (in blue boxes) observations of PSR B0740-28. We zoom in the area where the arc can be seen. The best-fitted results for arc structures are shown with red-dash curves.

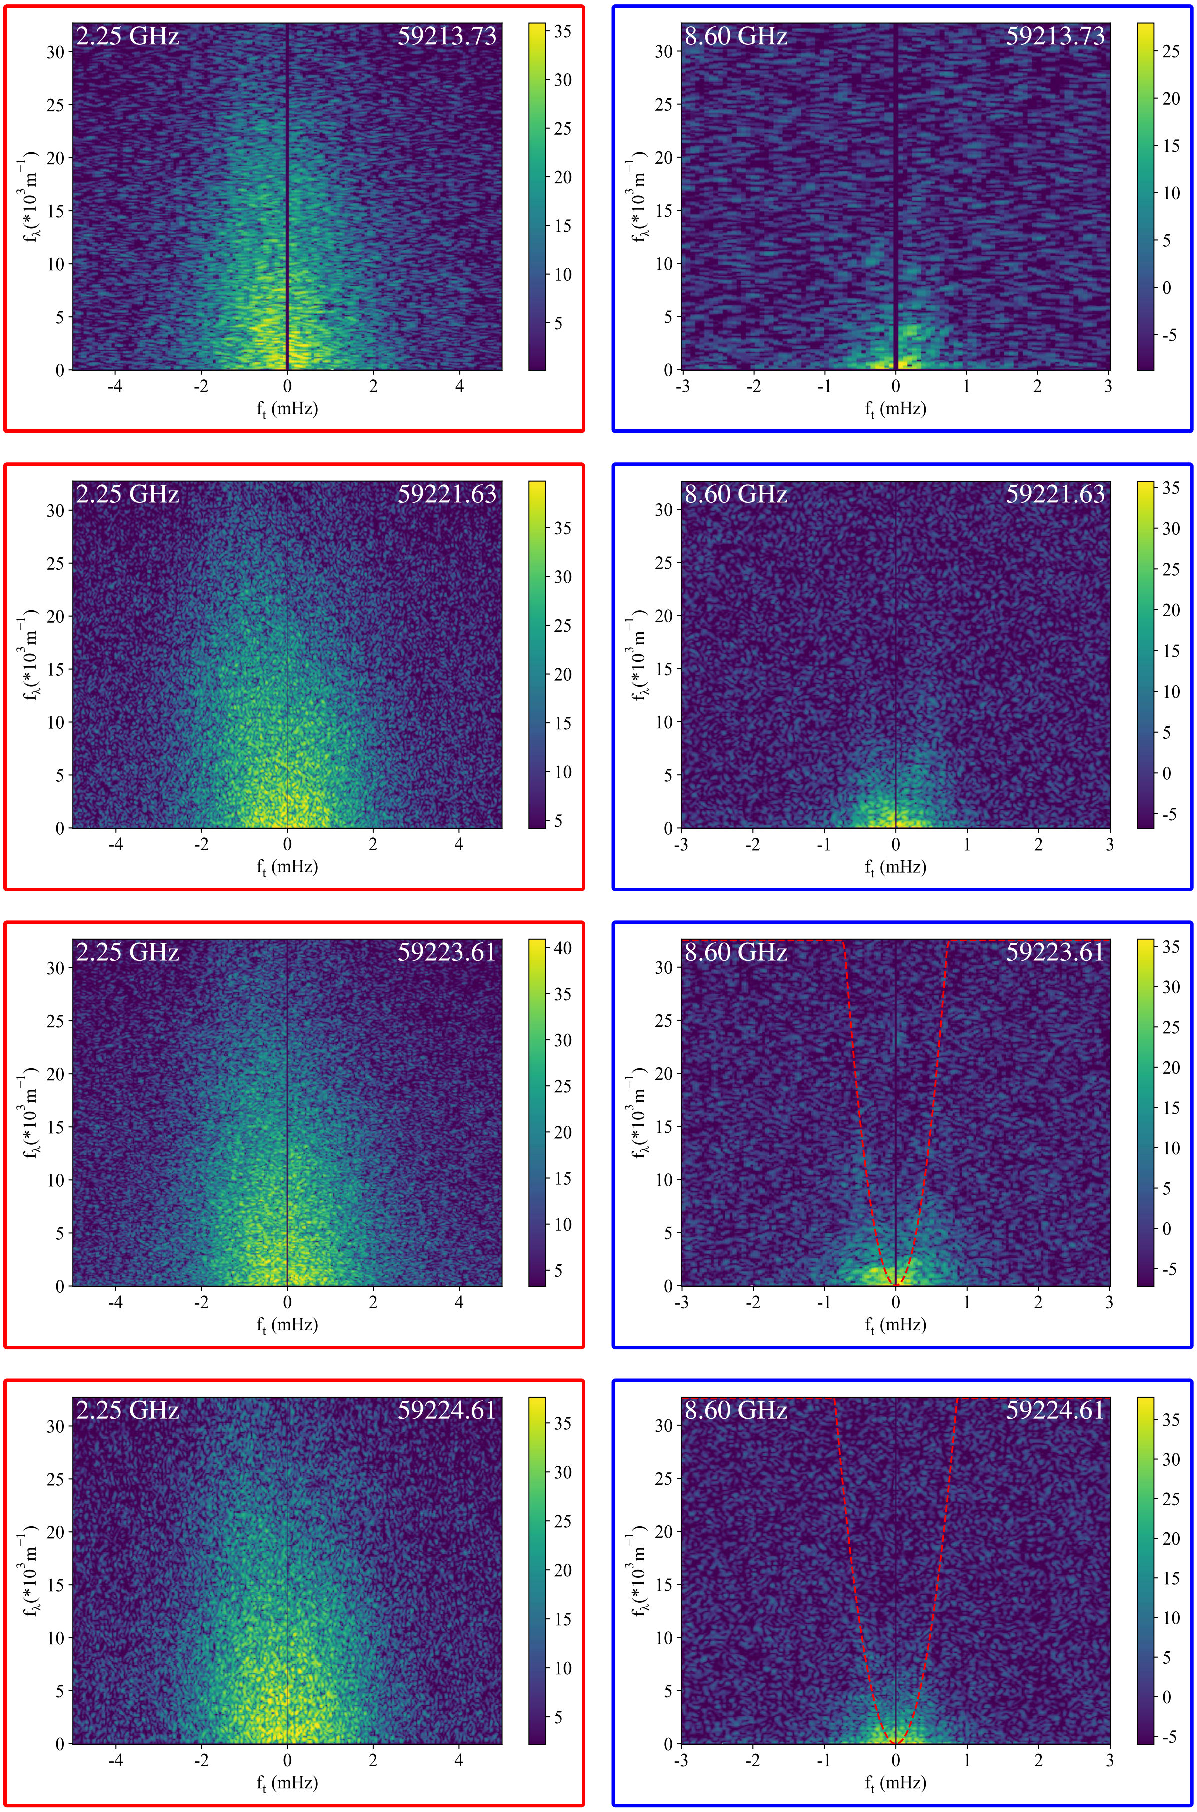


**Fig. S3** -continue

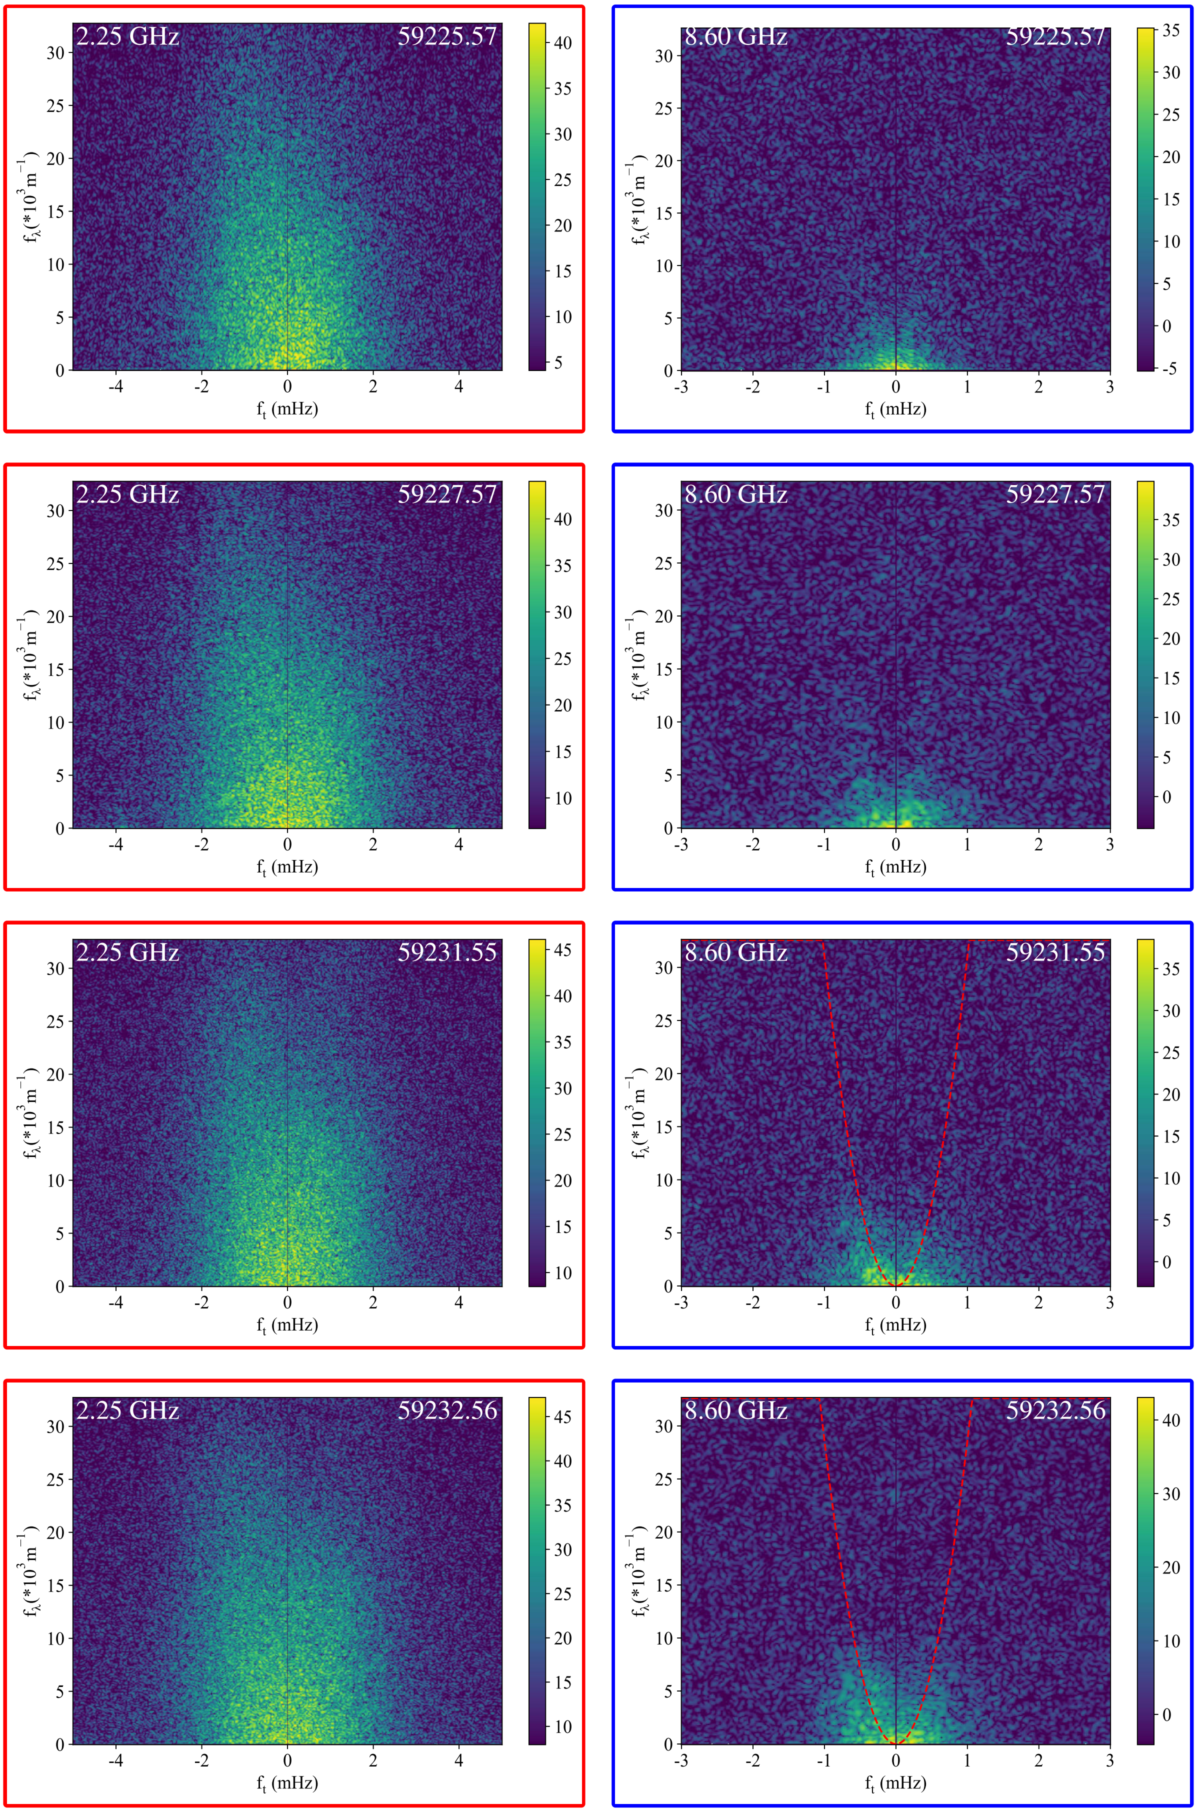


**Fig. S3** -continue

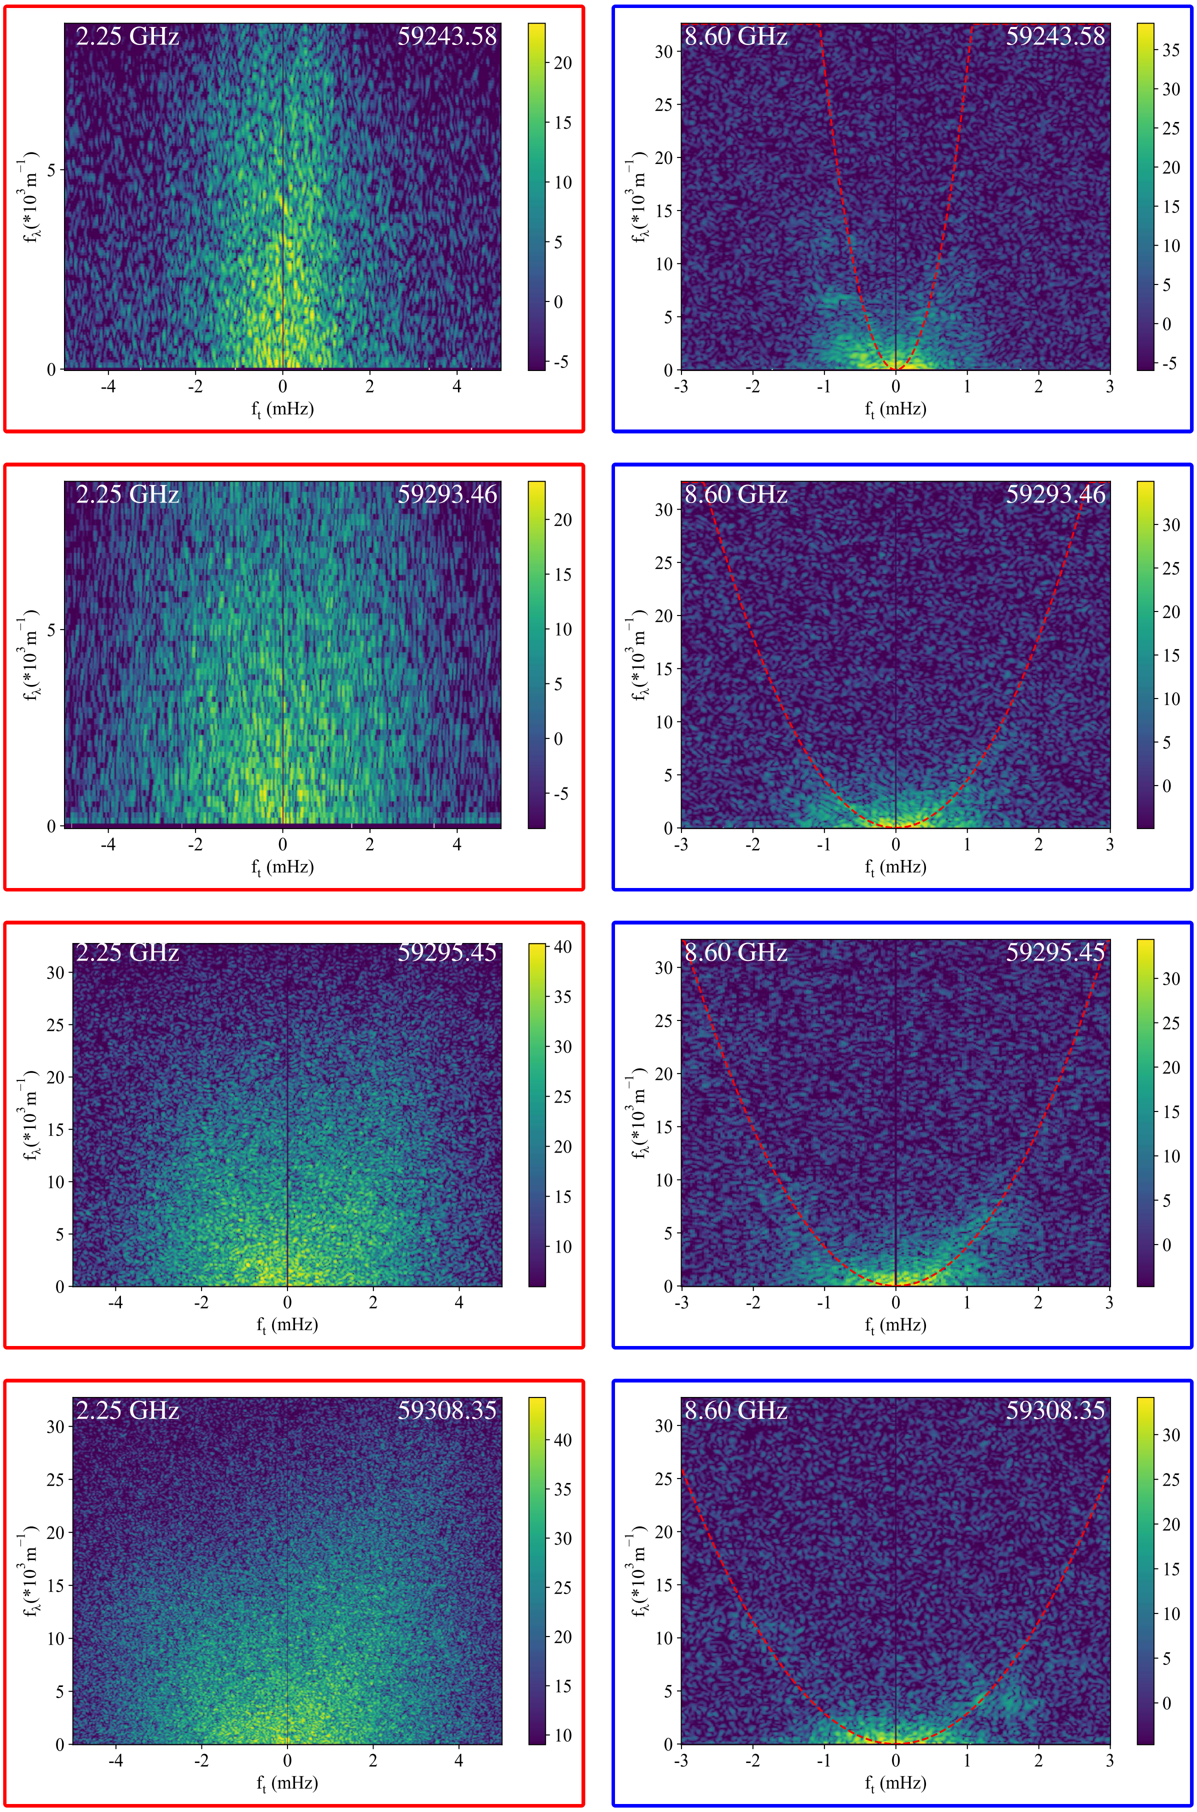


**Fig. S3** -continued

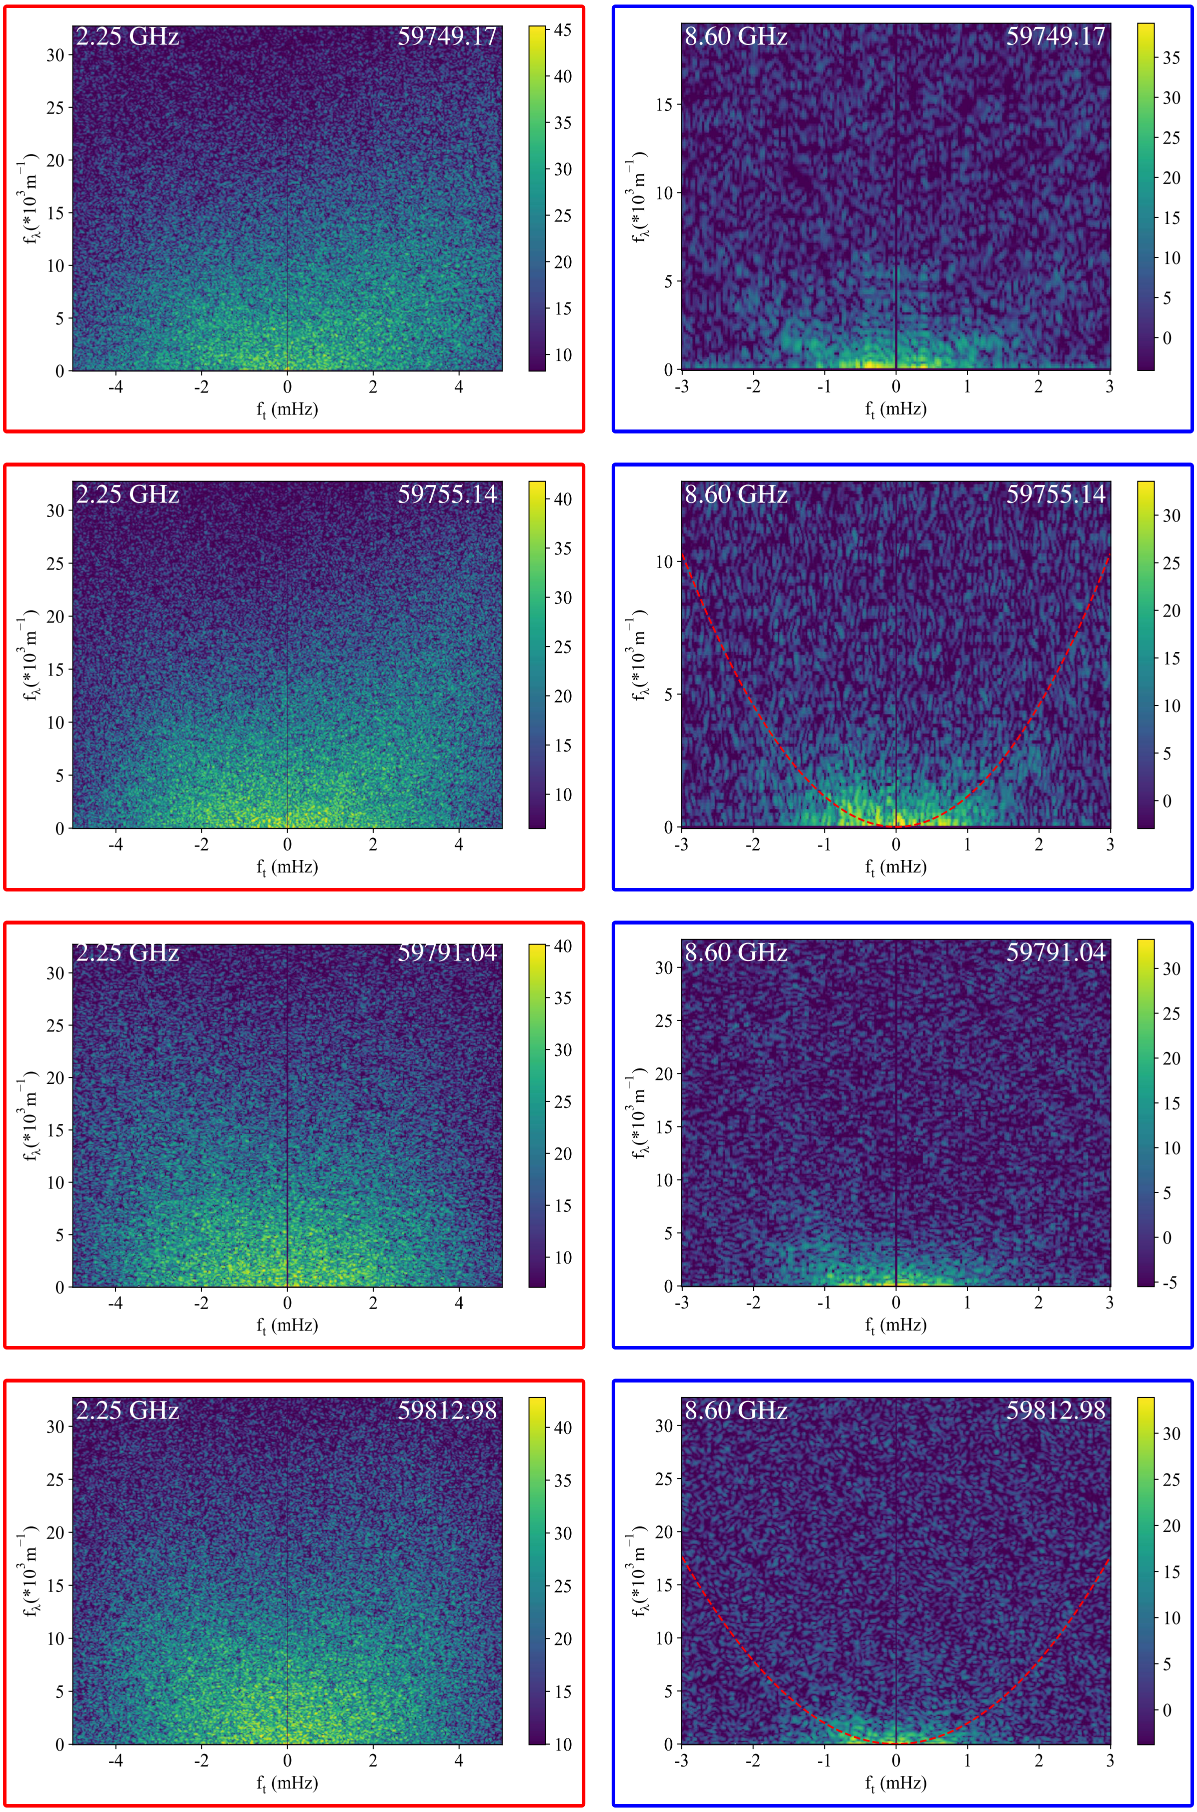


**Fig. S3** -continued

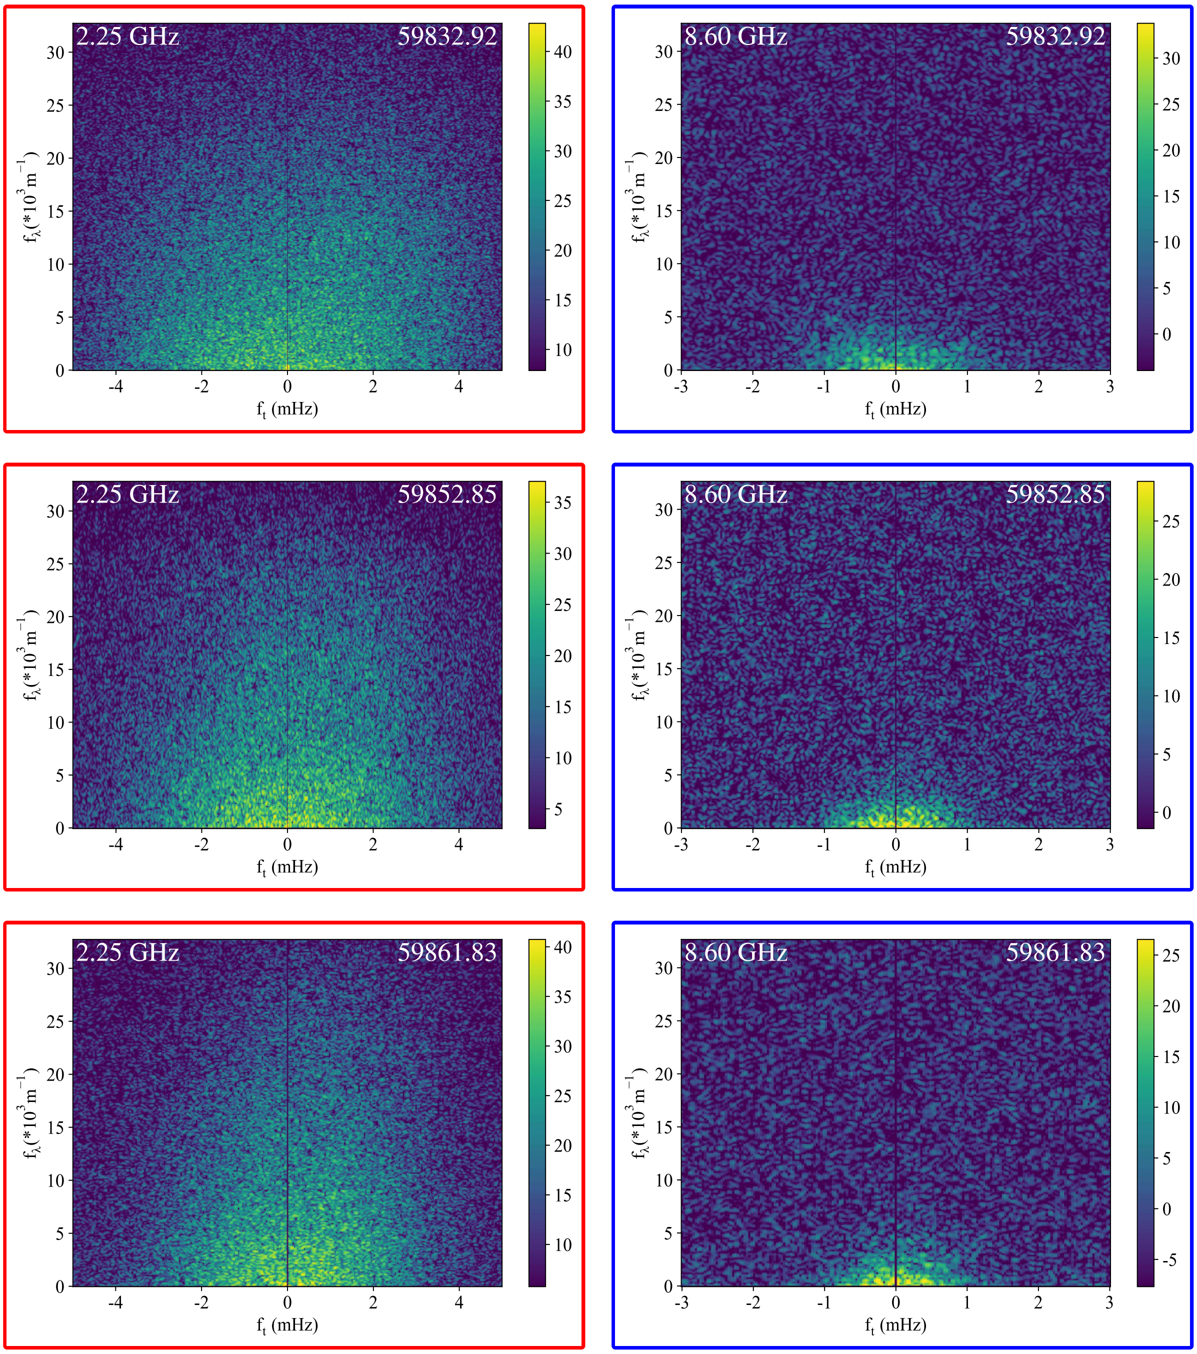


**Fig. S3** -continued

## S4. The normalized secondary spectra, the Doppler profiles and the mean power of Doppler profiles

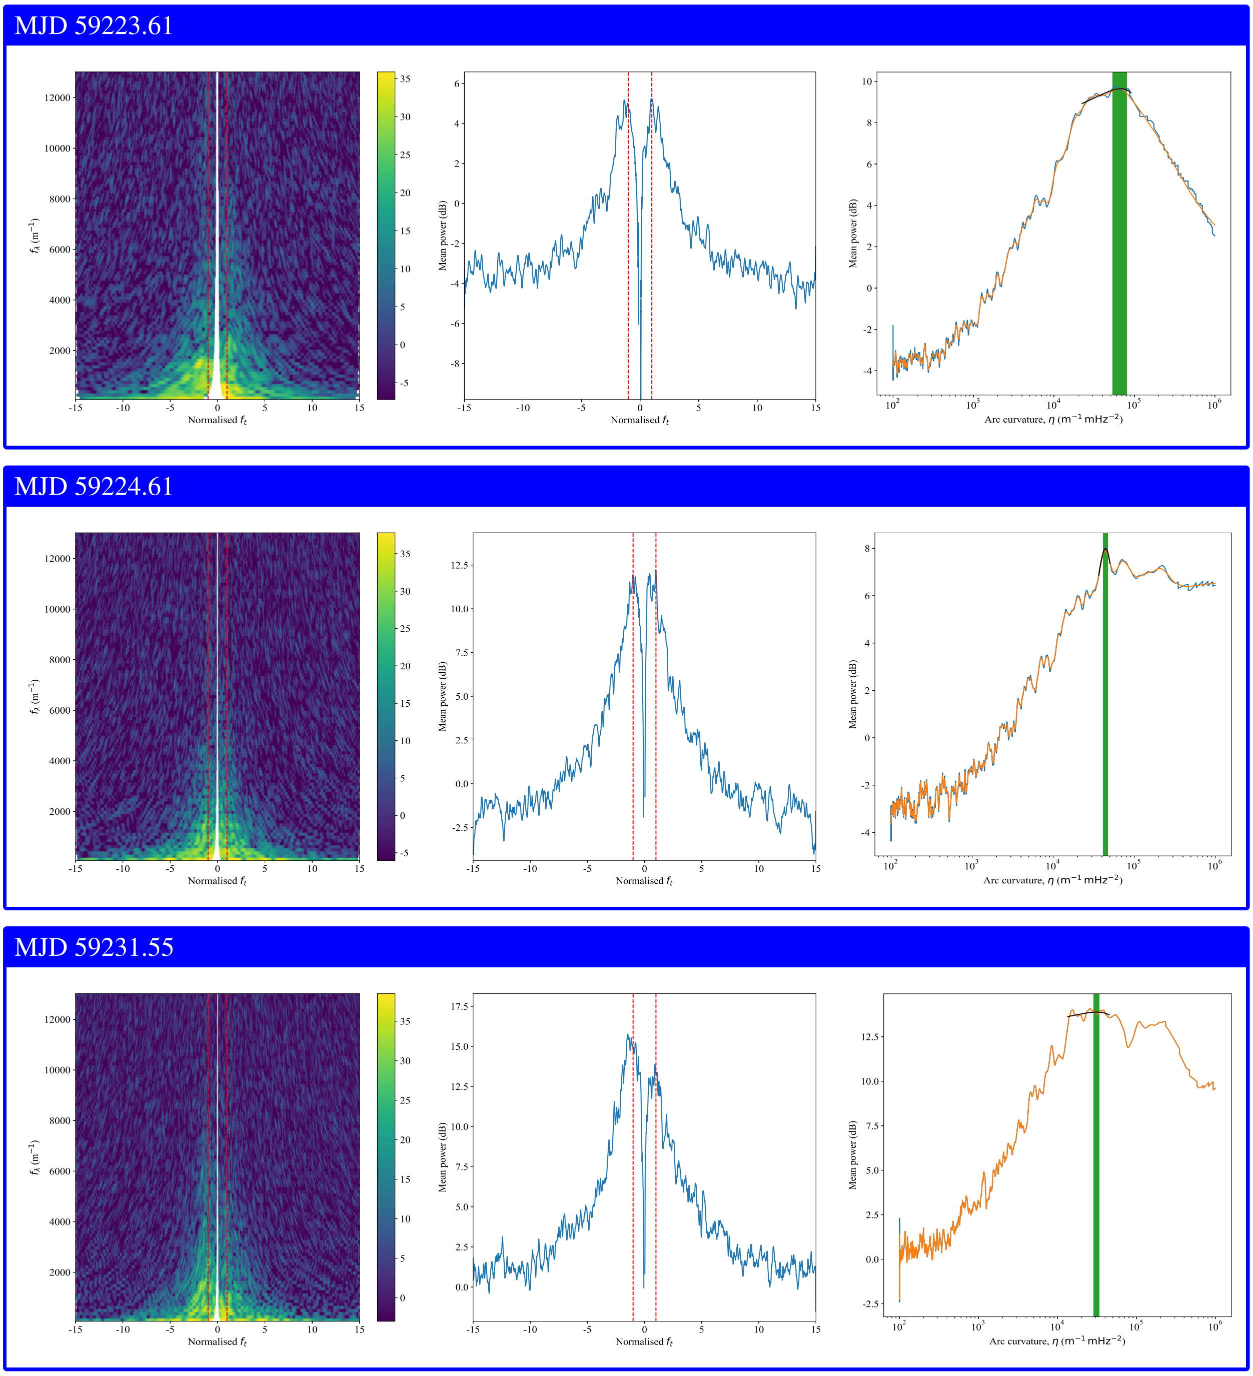


**Fig. S4** The normalized secondary spectra (left panel), the Doppler profiles (center panel), and the mean power of Doppler profiles as a function of arc curvature (right panel). The vertical red dashed lines indicated the arcs in normalized secondary spectra and the Doppler profiles. The green bands are the error range of arc curvature.

MJD 59232.56

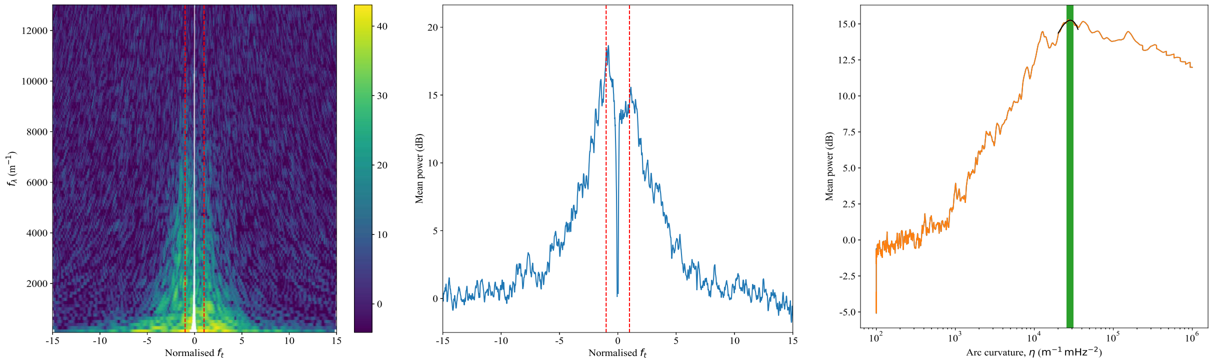


MJD 59243.58

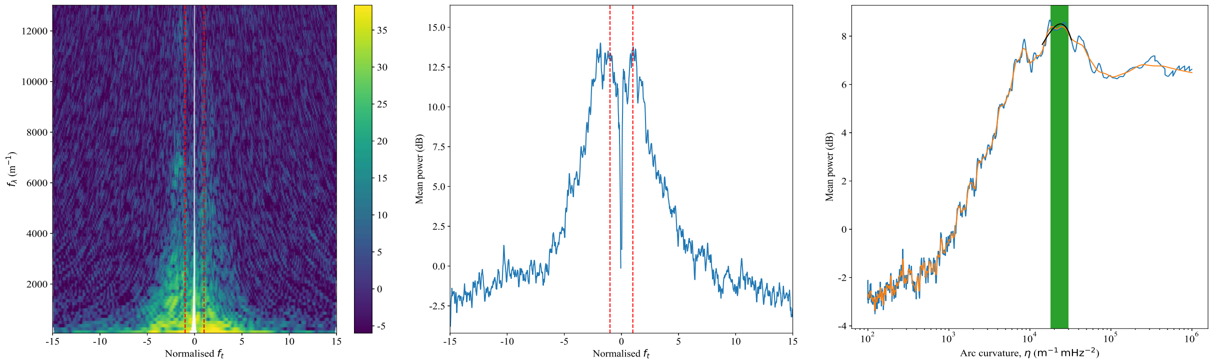


MJD 59293.46

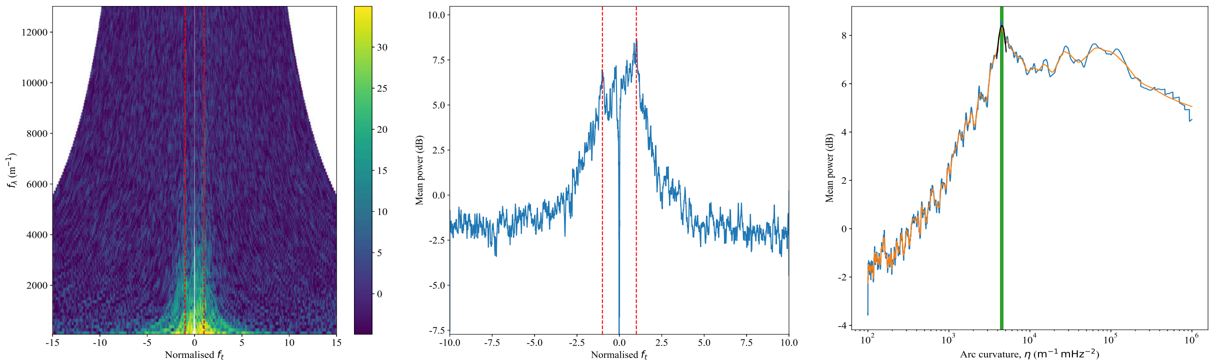


MJD 59295.45

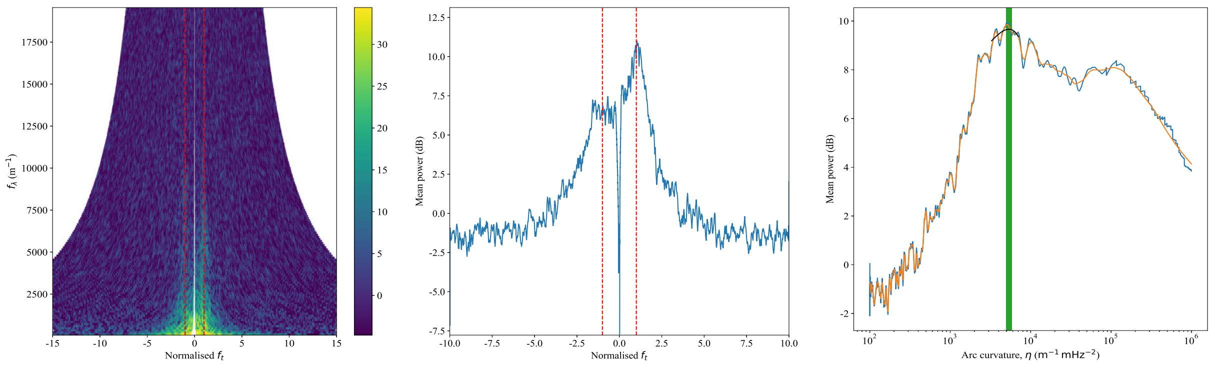


**Fig. S4** -continued

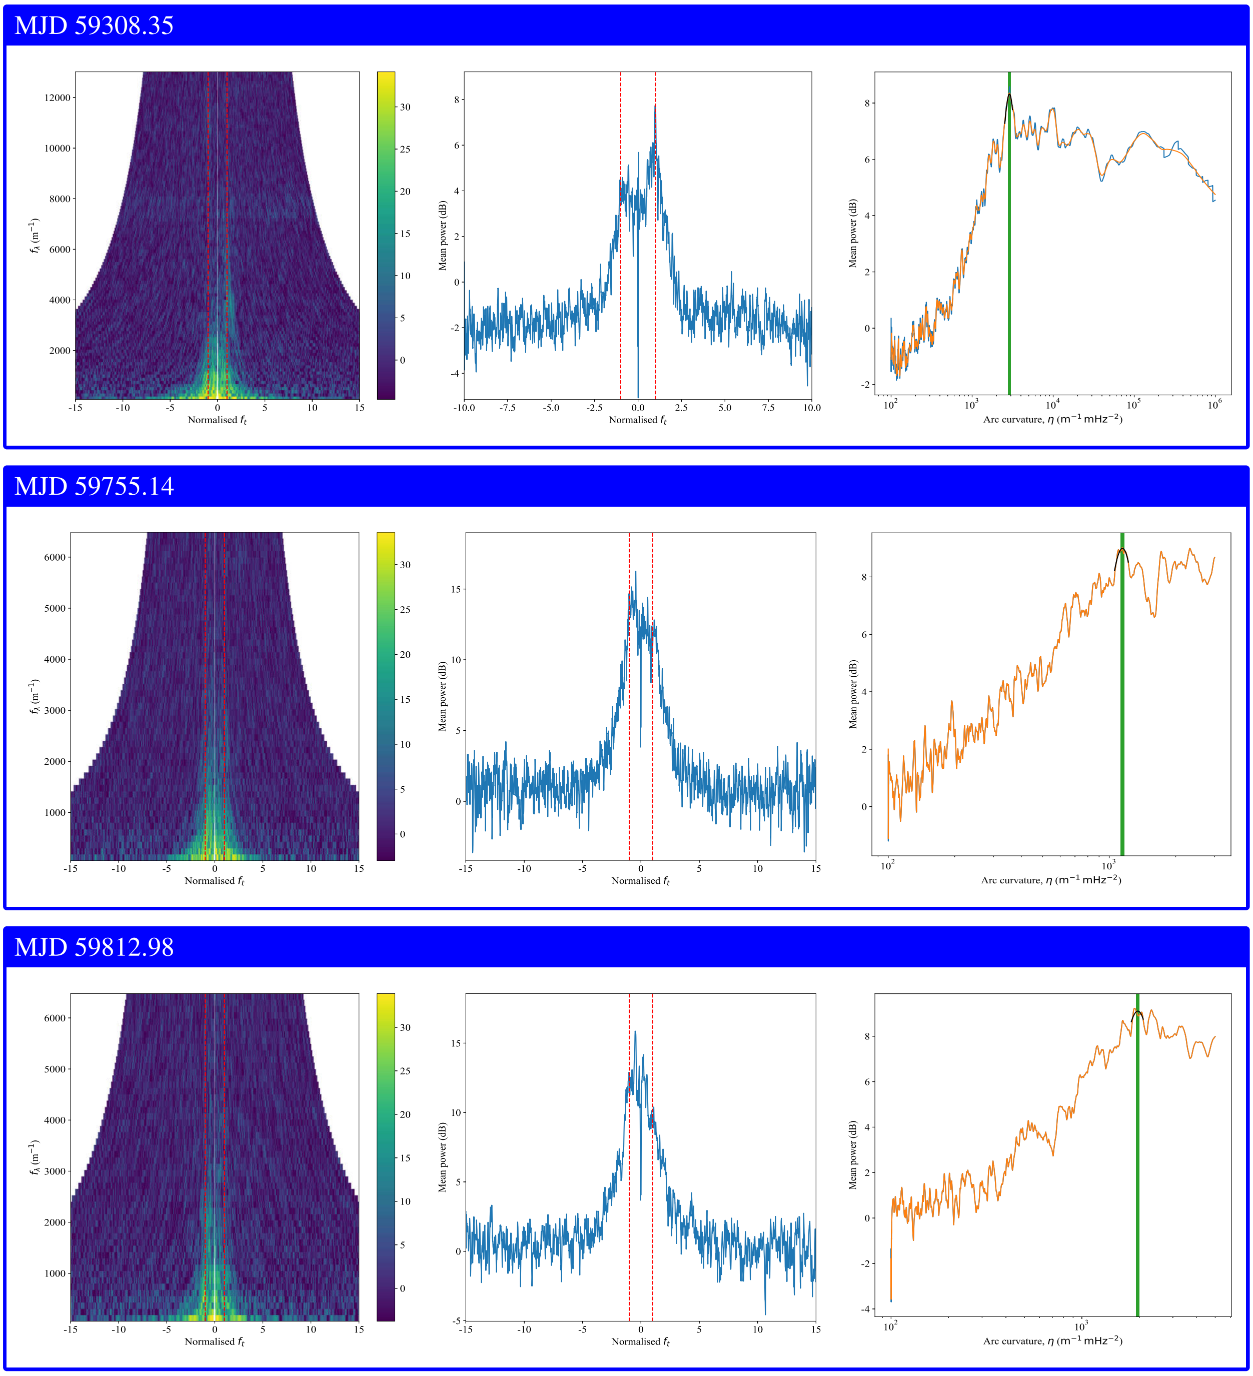


**Fig. S4** -continue
